# Supplementary material for: Observation of the decay $ \Lambda_b^0\rightarrow \Lambda_c^+\tau^-\overline{\nu}_{\tau}$
Source: arXiv:2201.03497 source file (2023-03-01)
Supplement: Supplementary file 1 [file supplementary-app.tex]

\section*{Supplementary material}
\begin{figure}[h]
    \centering
    \includegraphics[width=0.8\textwidth]{../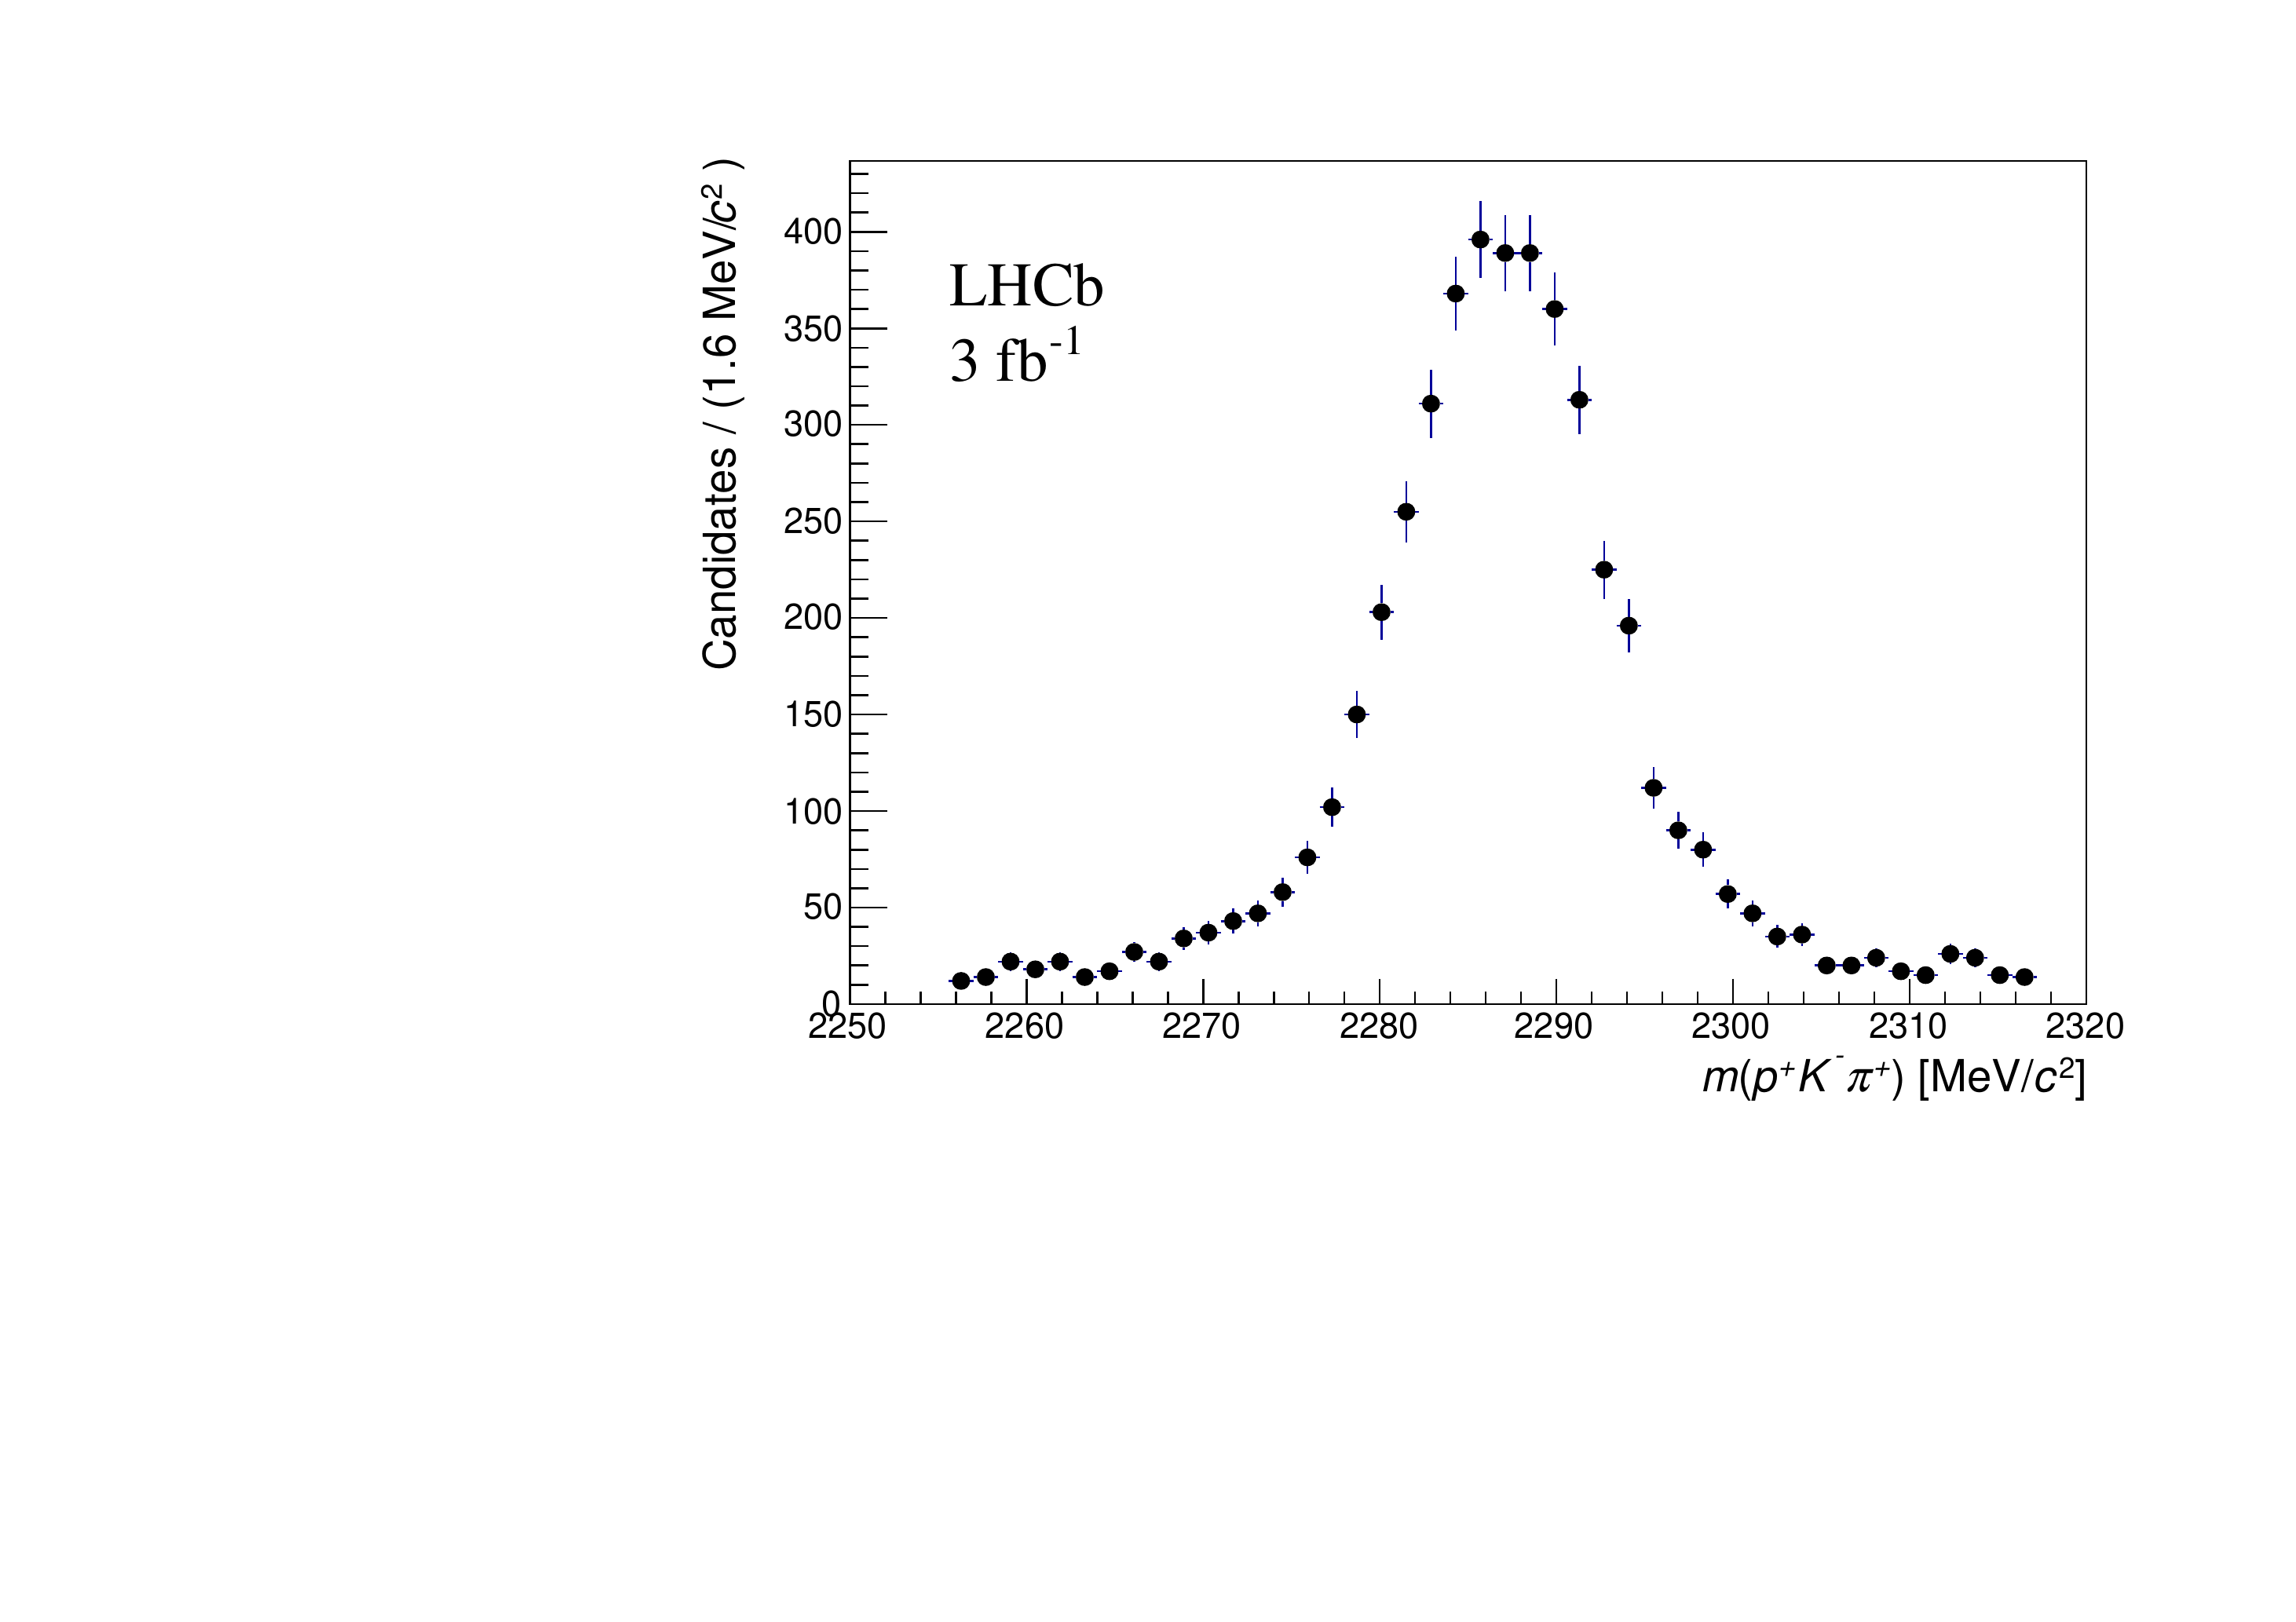}
        \caption{
    \small %captions should be a little bit smaller than main text
Distribution of the p\Km\pip invariant mass for all \Lb\to\Lc\taum\neutb candidates in the final fit sample.}
  \label{figsupp:lcmass}
\end{figure}
\begin{figure}[h]
    \centering
        \includegraphics[width=0.8\textwidth]{../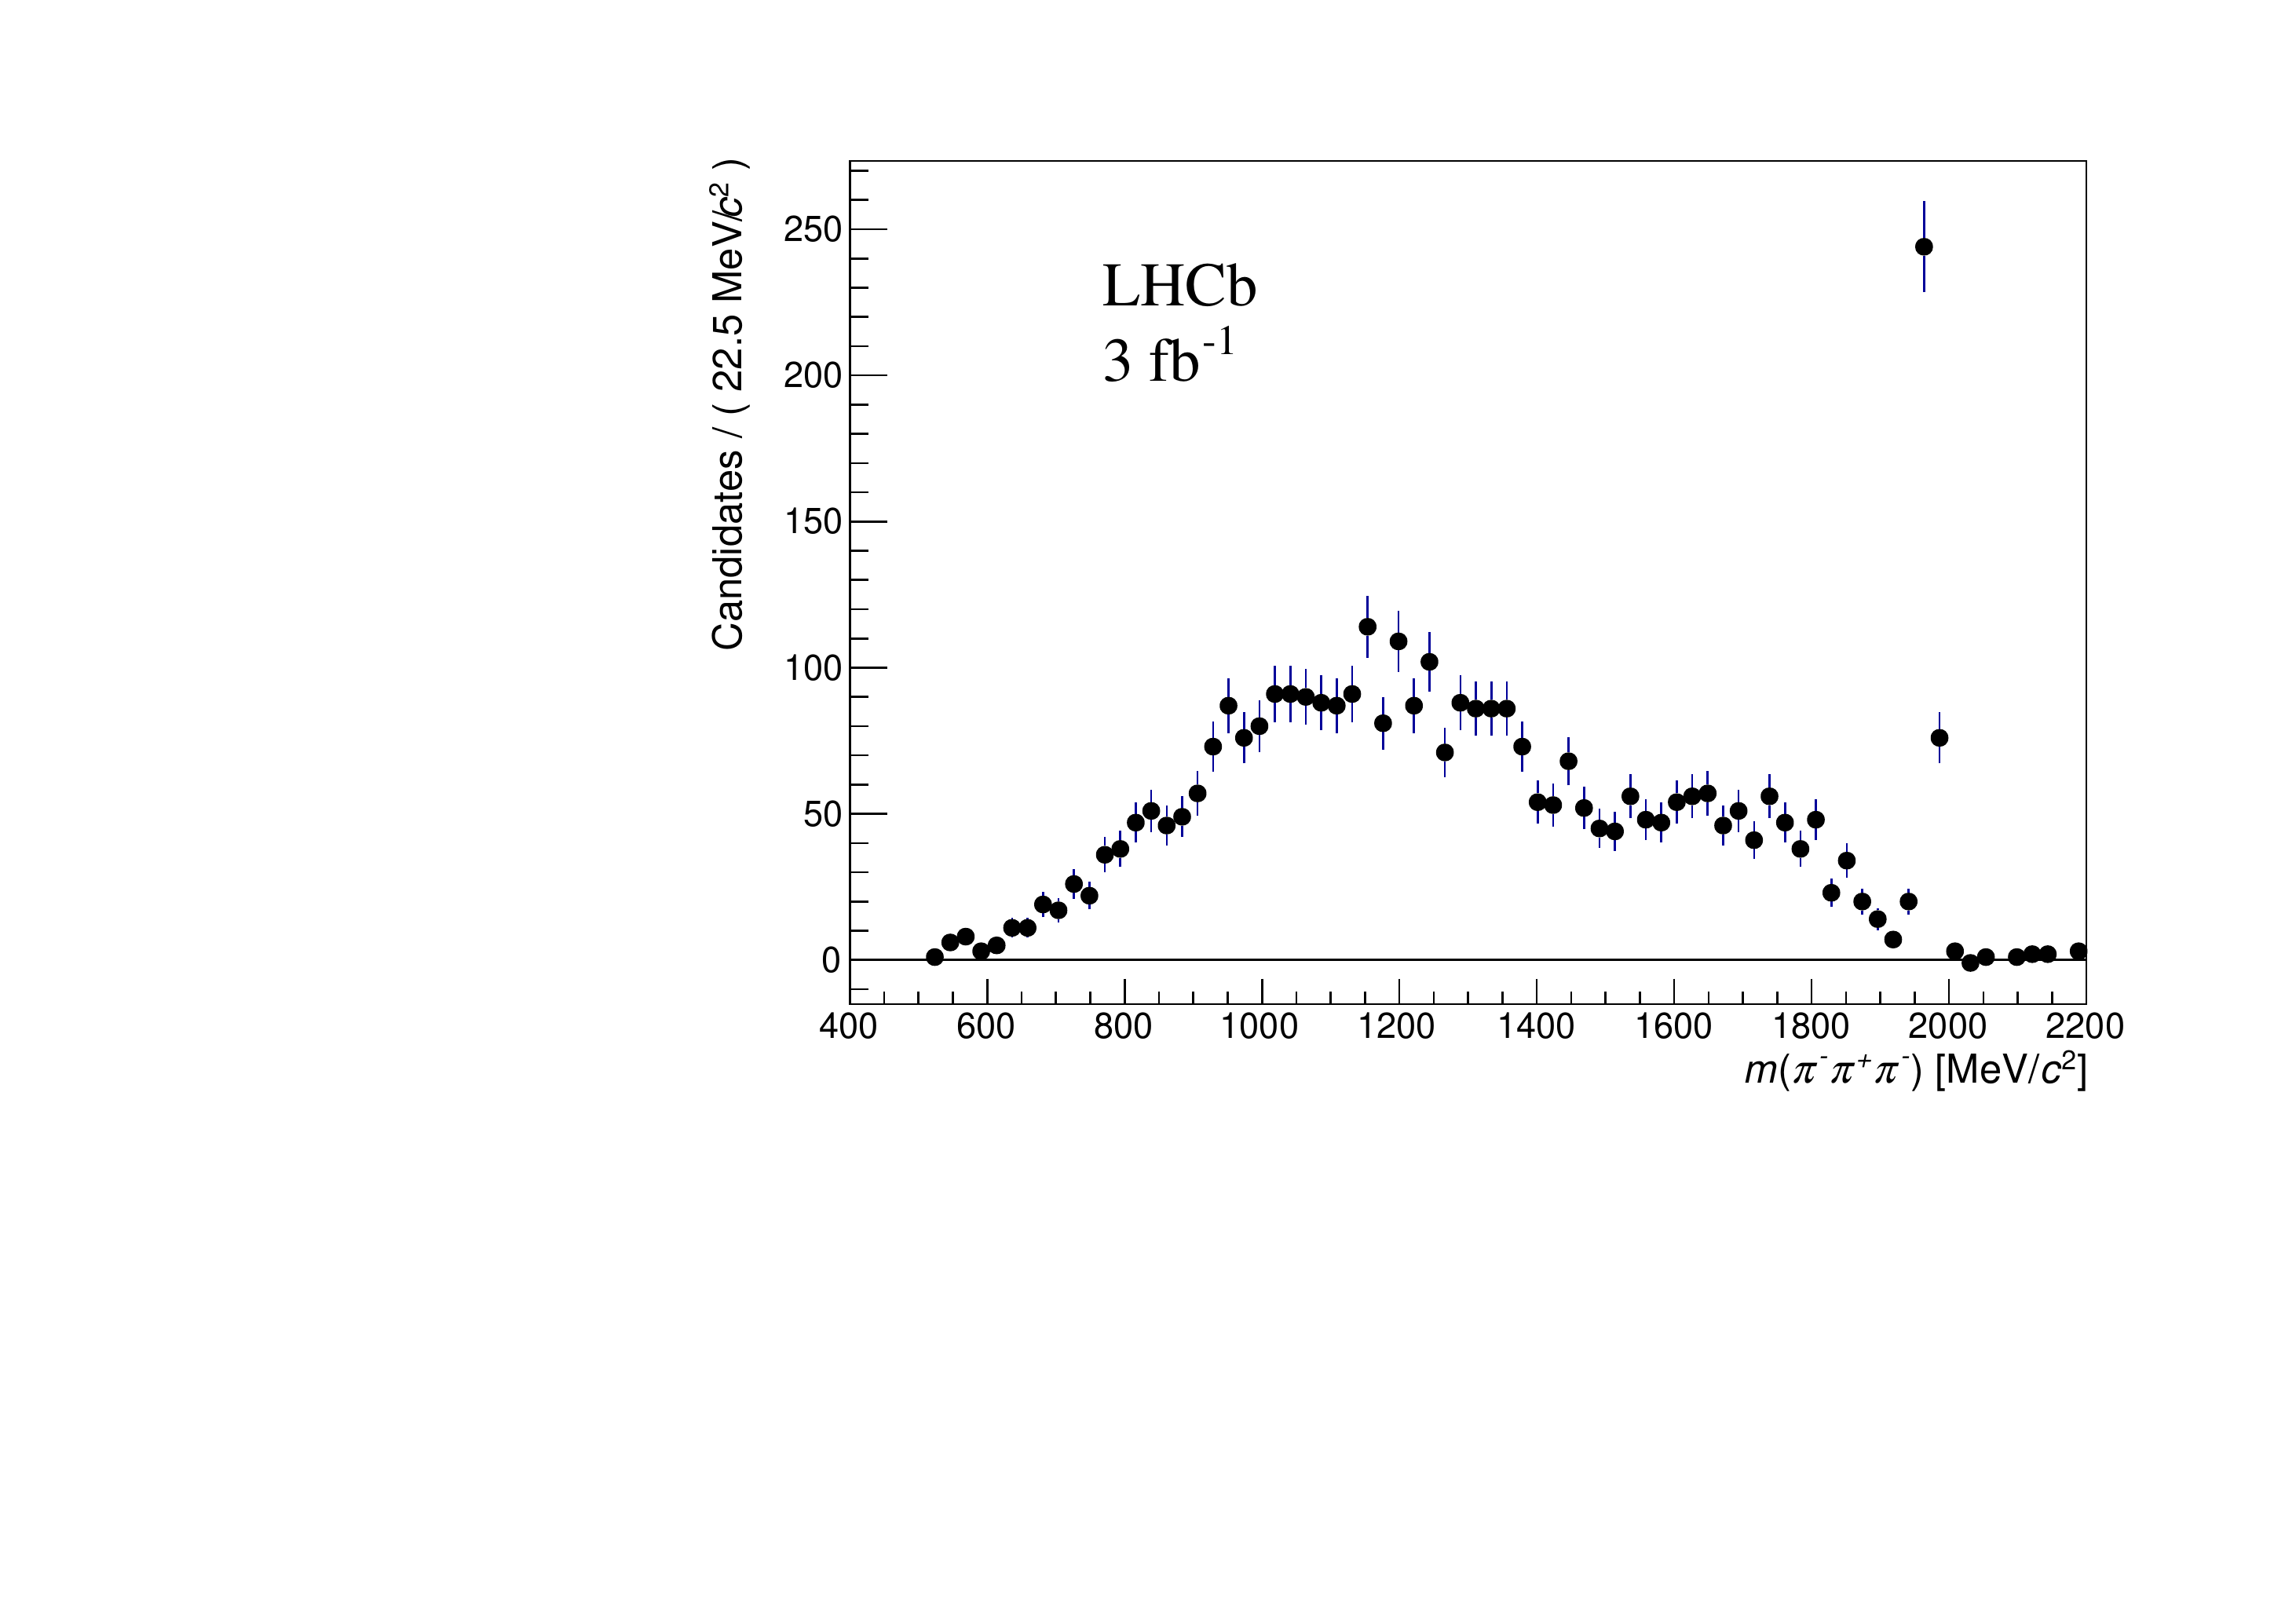}
        \caption{
    \small %captions should be a little bit smaller than main text
Distribution of the \pim\pip\pim invariant mass for all \Lb\to\Lc\taum\neutb candidates after  the \Lc sideband subtraction passing the inverted topology requirement.}
  \label{figsupp:3pimass}
\end{figure}
\begin{figure}[h]
    \centering
        \includegraphics[width=0.8\textwidth]{../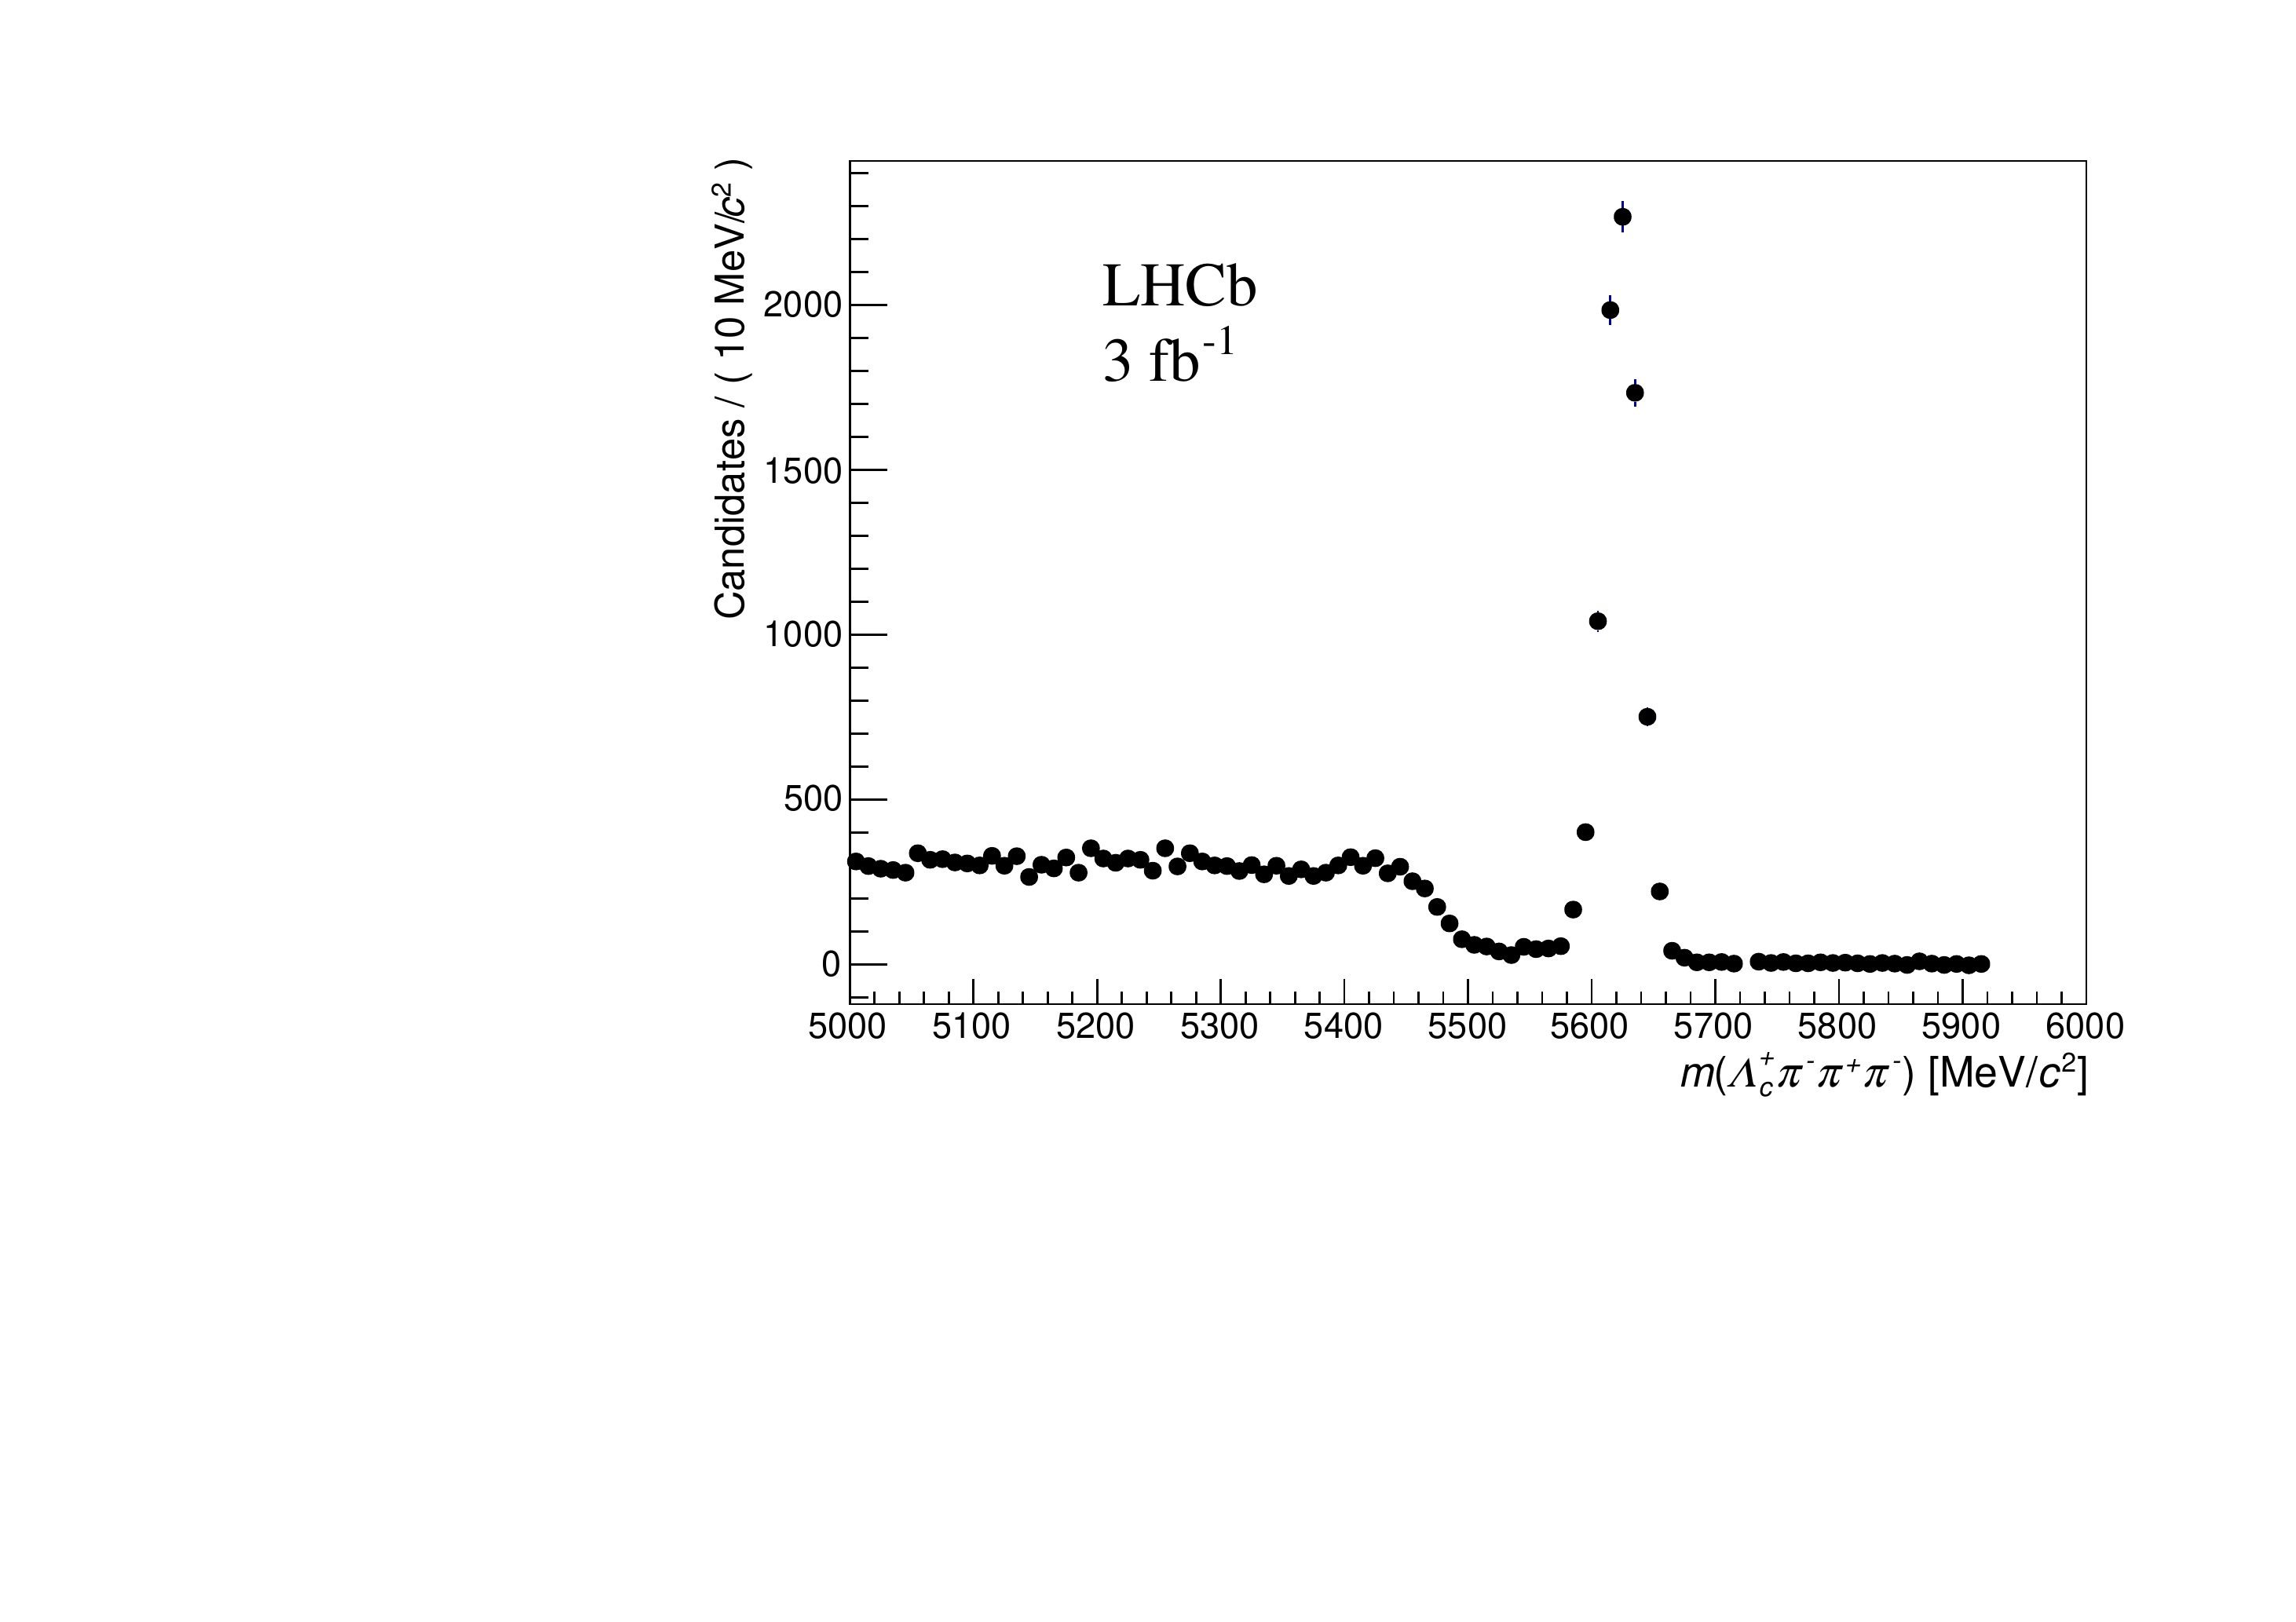}
        \caption{
    \small %captions should be a little bit smaller than main text
Distribution of the \Lc\pim\pip\pip invariant mass for all \Lb\to\Lc\taum\neutb candidates  after  the \Lc sideband subtraction.}
  \label{figsupp:lbmass}
\end{figure}
\begin{figure}[h]
    \centering
        \includegraphics[width=0.8\textwidth]{../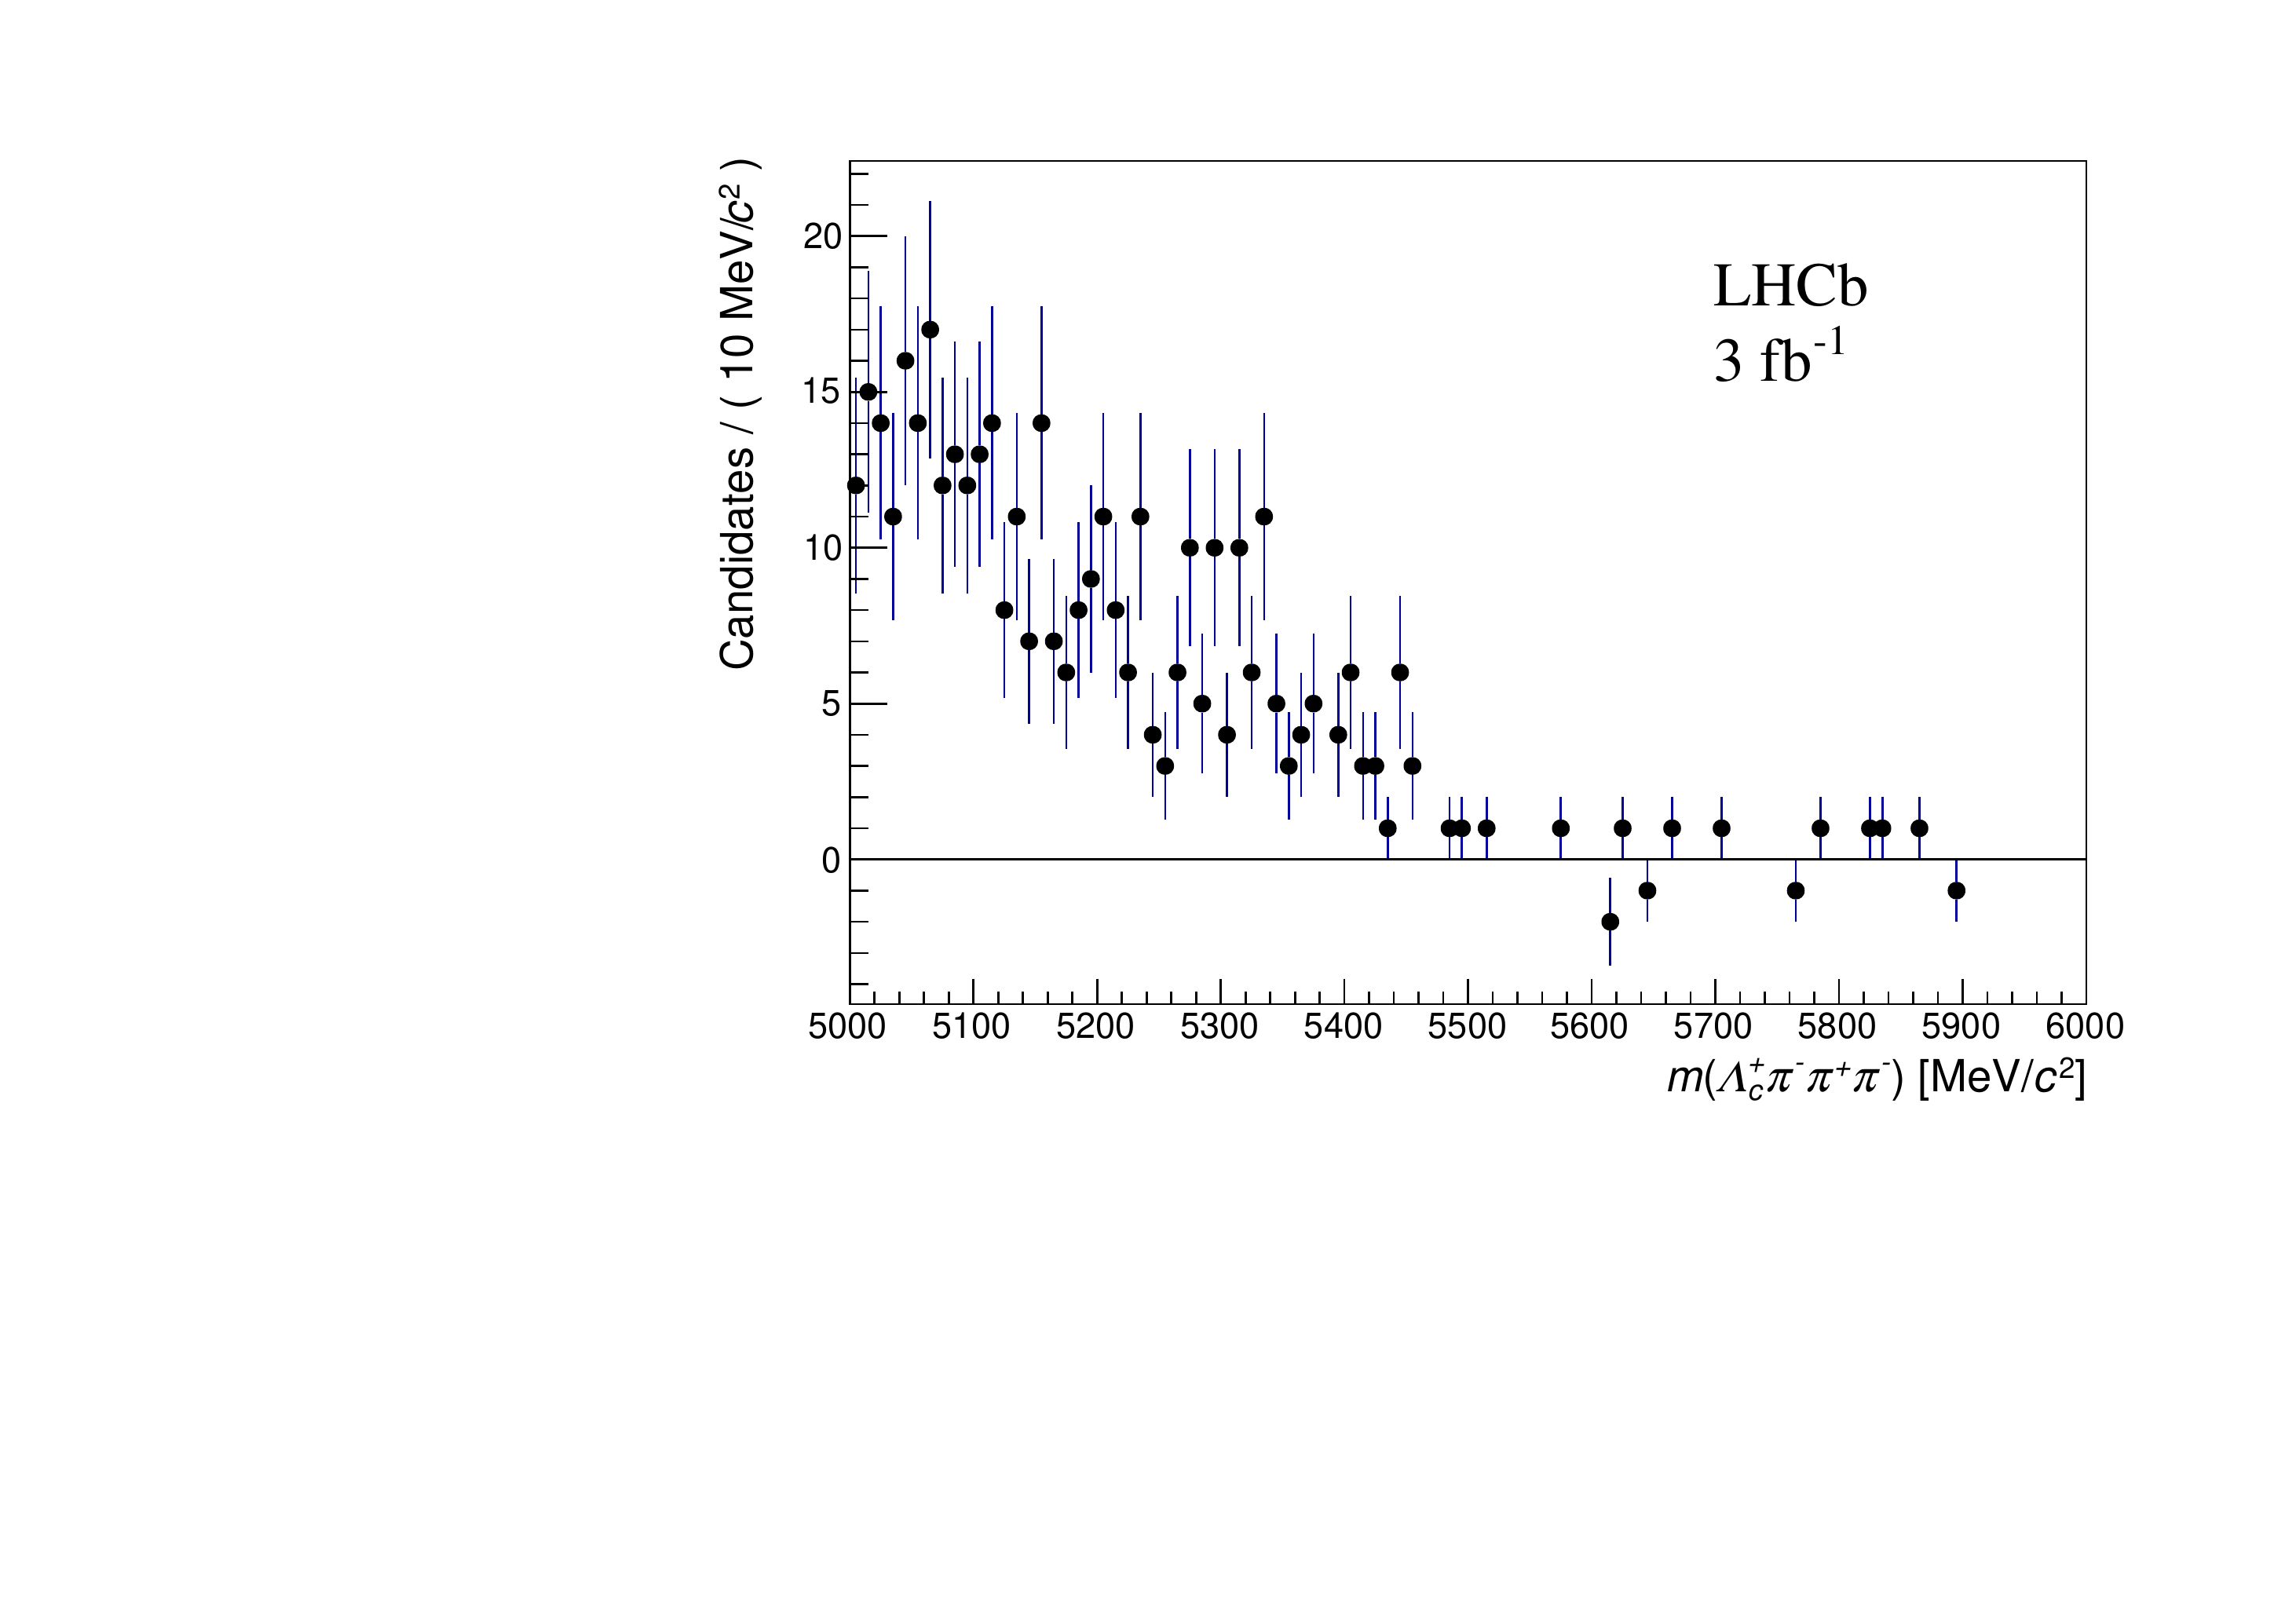}
        \caption{
    \small %captions should be a little bit smaller than main text
Distribution of the \Lc\pim\pip\pip invariant mass for all \Lb\to\Lc\taum\neutb candidates  after  the \Lc sideband subtraction passing the inverted vertex topology requirement.}
  \label{figsupp:lbmass_aftertopo}
\end{figure}

\begin{figure}[h]
    \centering
        \includegraphics[width=0.8\textwidth]{../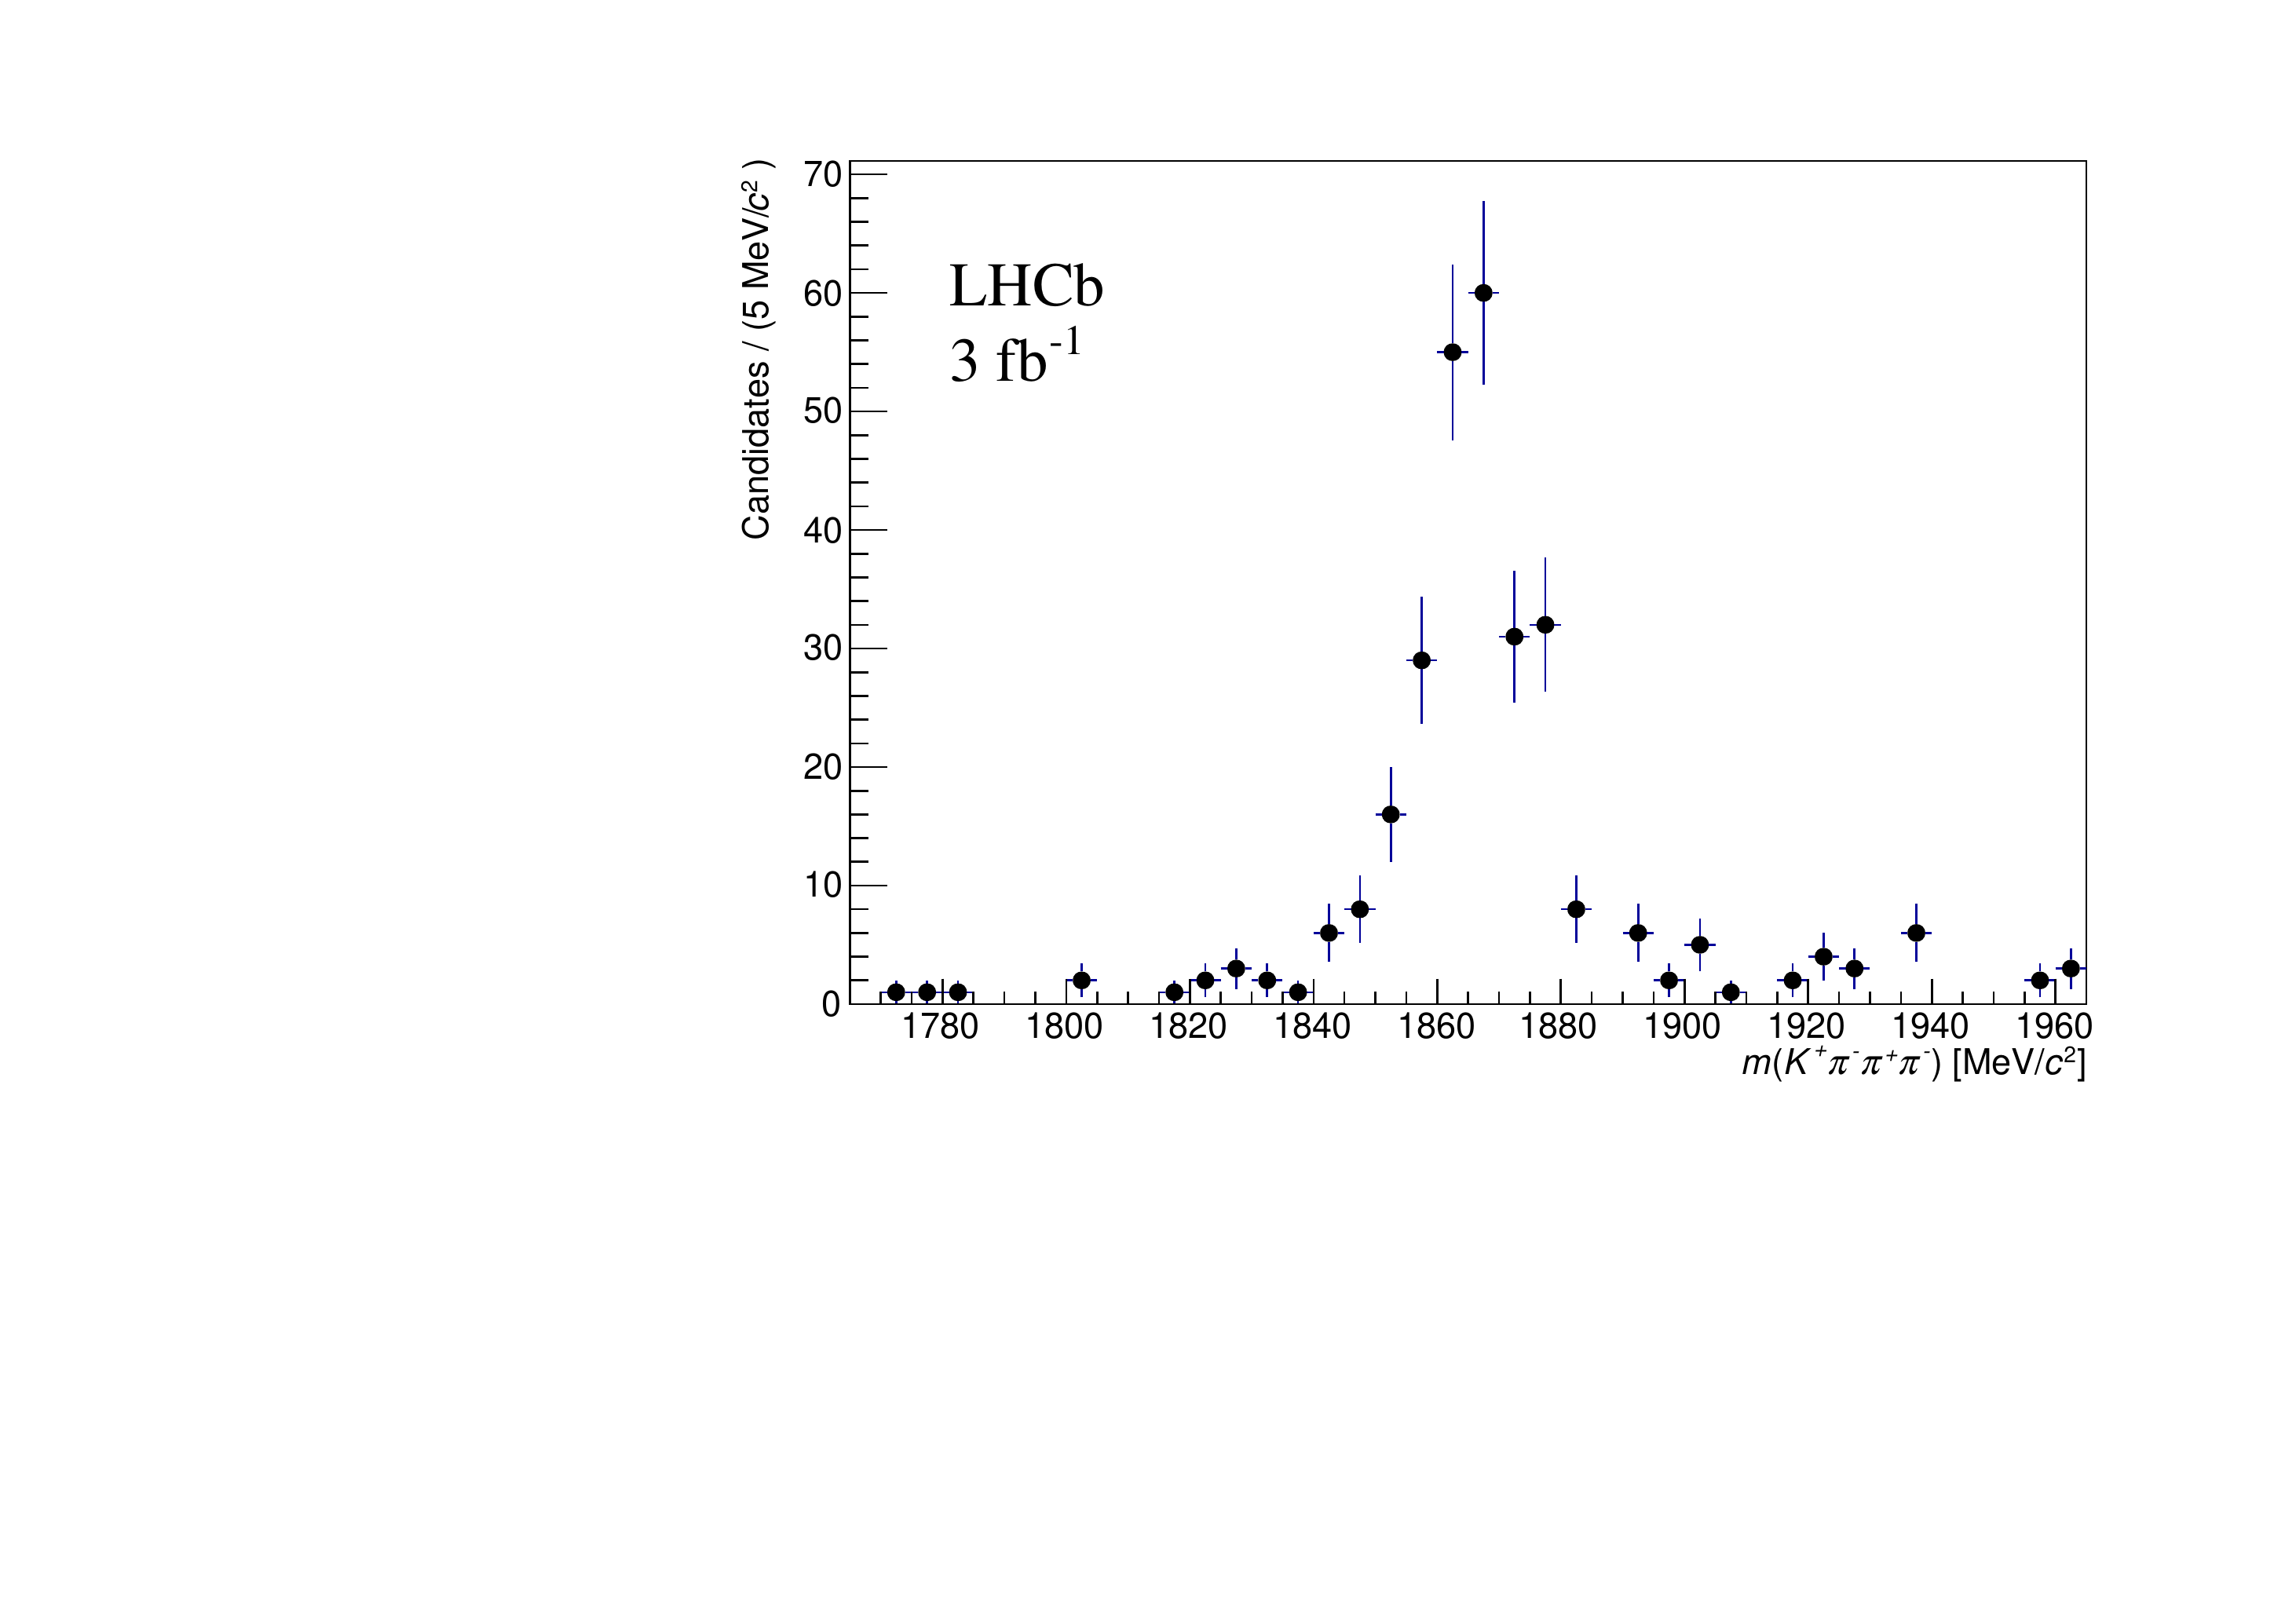}
        \caption{
    \small %captions should be a little bit smaller than main text
Distribution of the \Kp\pim\pip\pim invariant mass for all \Lb\to\Lc\Dzb$X$ candidates where a kaon track is found compatible with the 3\pion vertex.}
  \label{figsupp:D0mass}
\end{figure}
\begin{figure}[h]
    \centering
        \includegraphics[width=0.8\textwidth]{../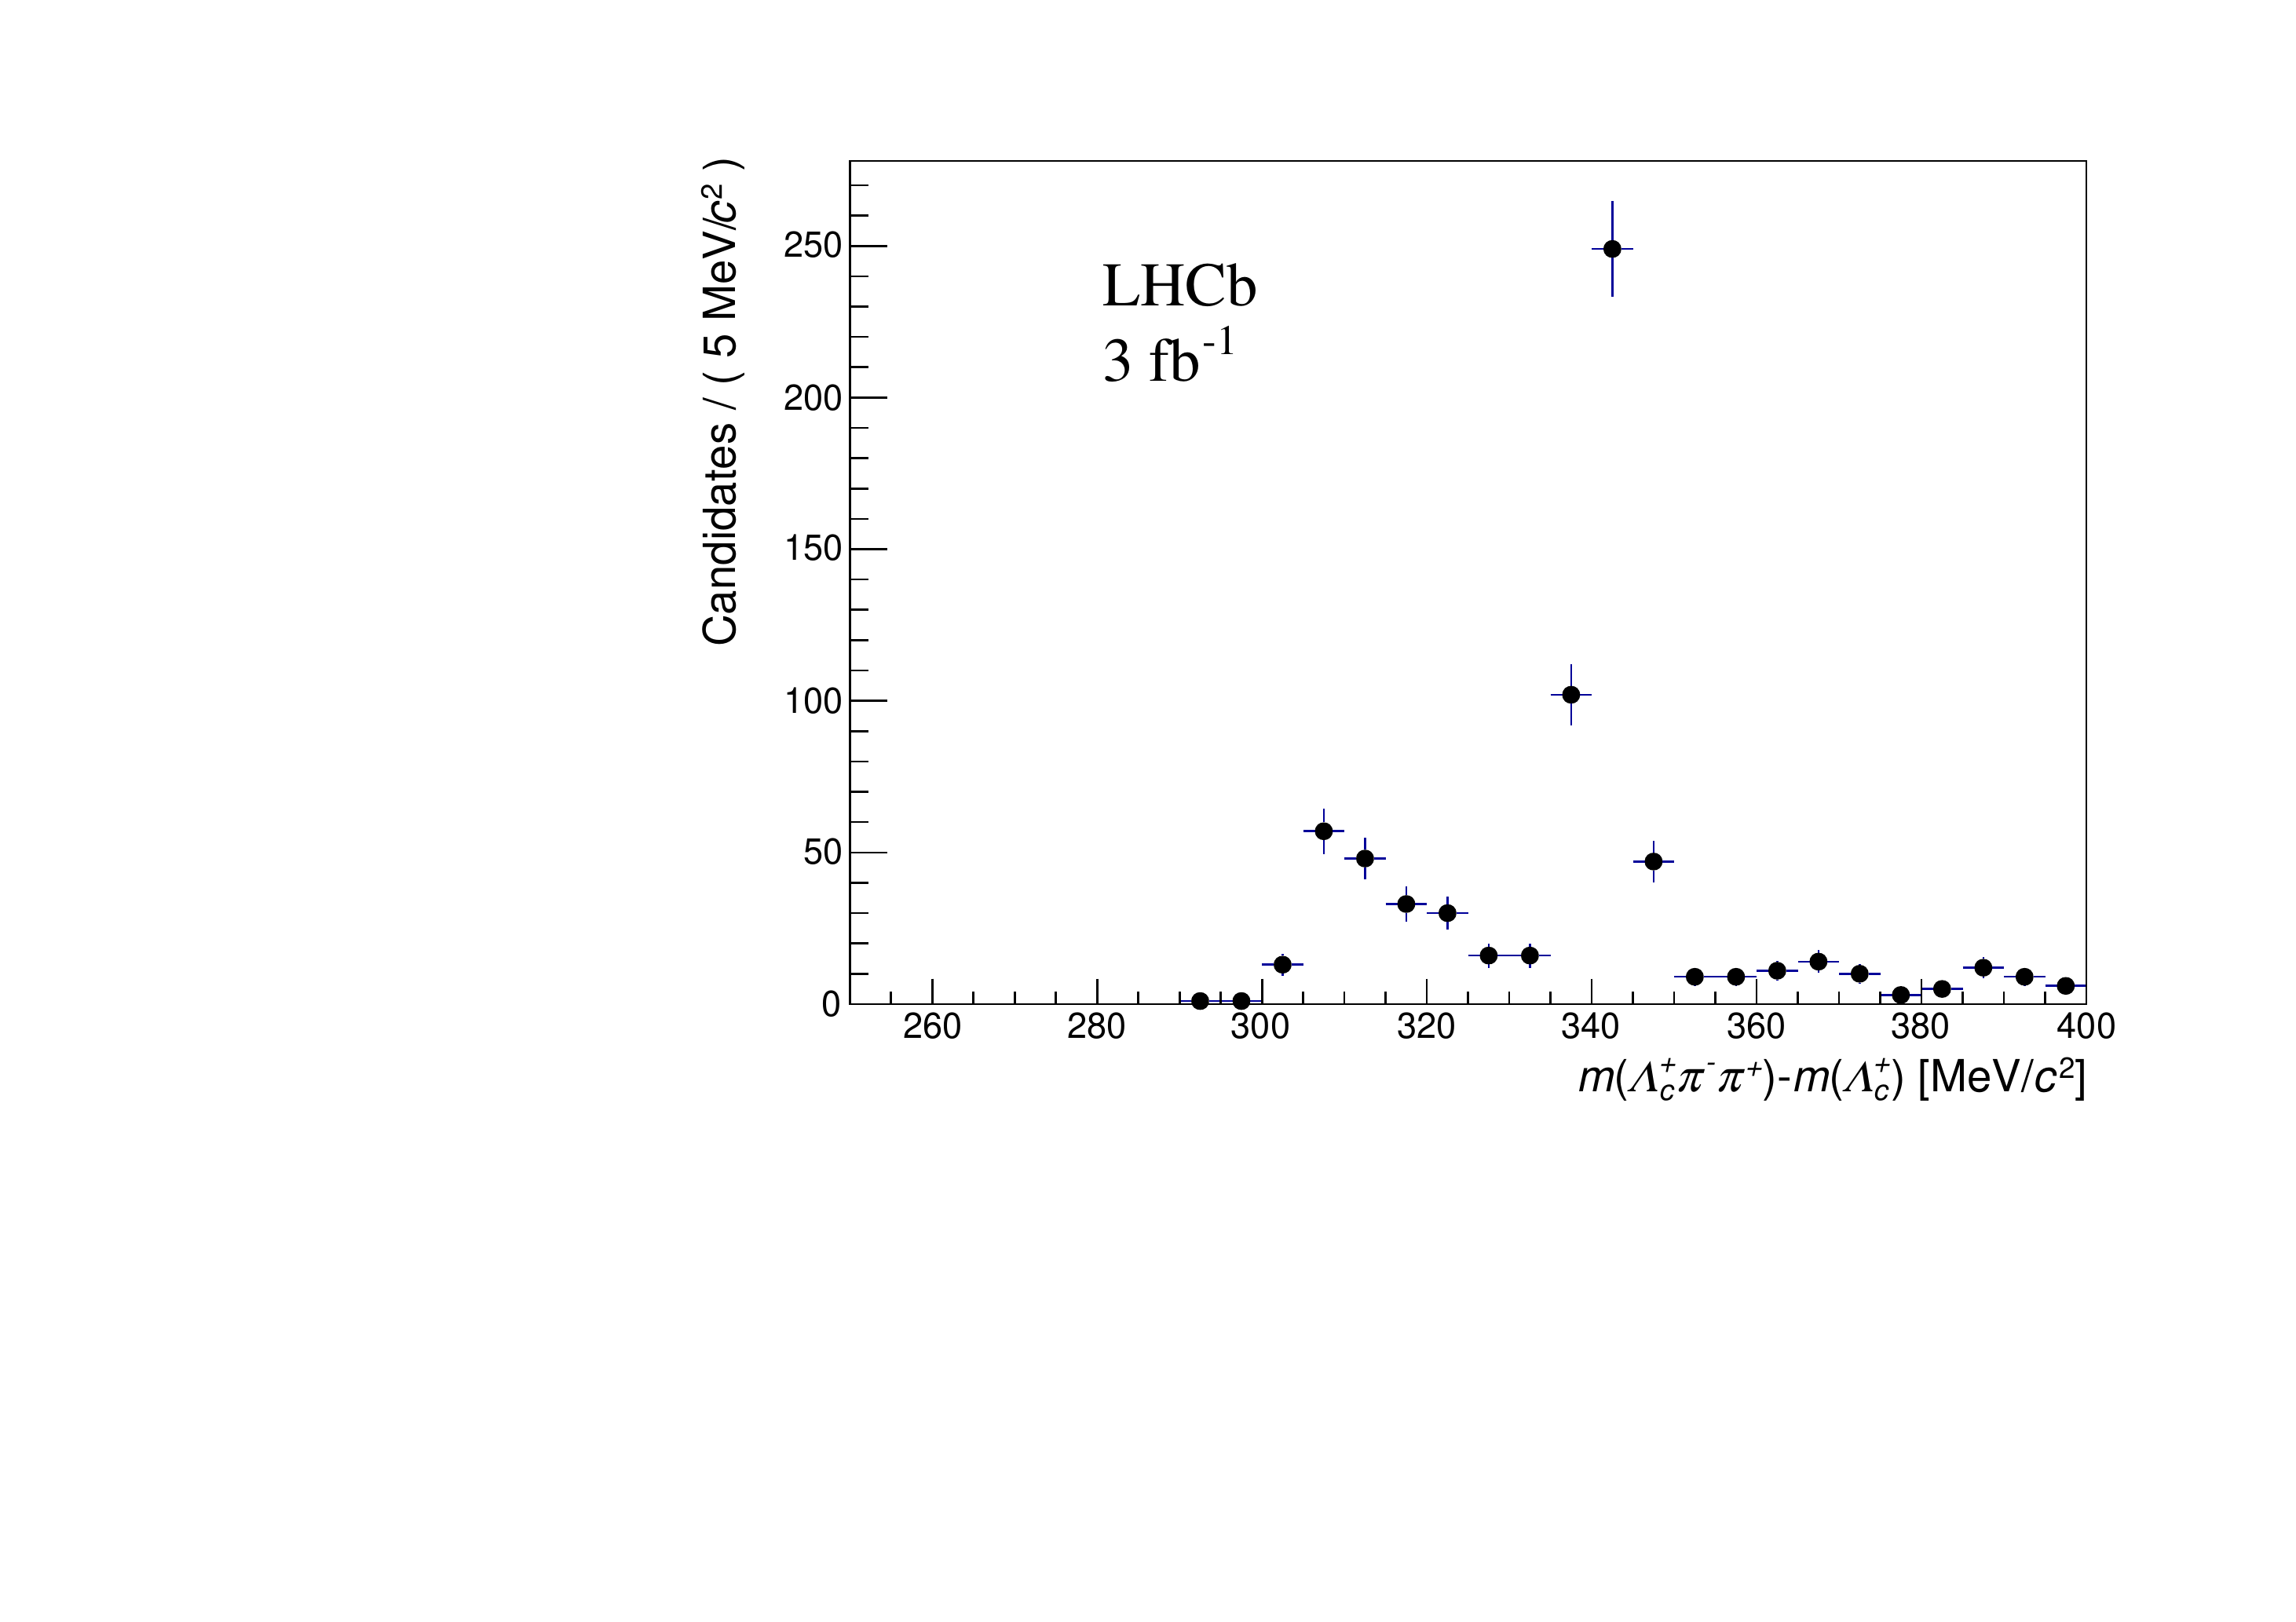}
        \caption{
    \small %captions should be a little bit smaller than main text
Distribution of the difference between \Lc\pim\pip invariant mass and the \Lc invariant mass for all candidates reconstructed in the \Lb\to\Lc\pim\pip\pim normalisation channel peak.}
  \label{figsupp:lcstar}
\end{figure}

\begin{figure}[h]
    \centering
        \includegraphics[width=0.8\textwidth]{../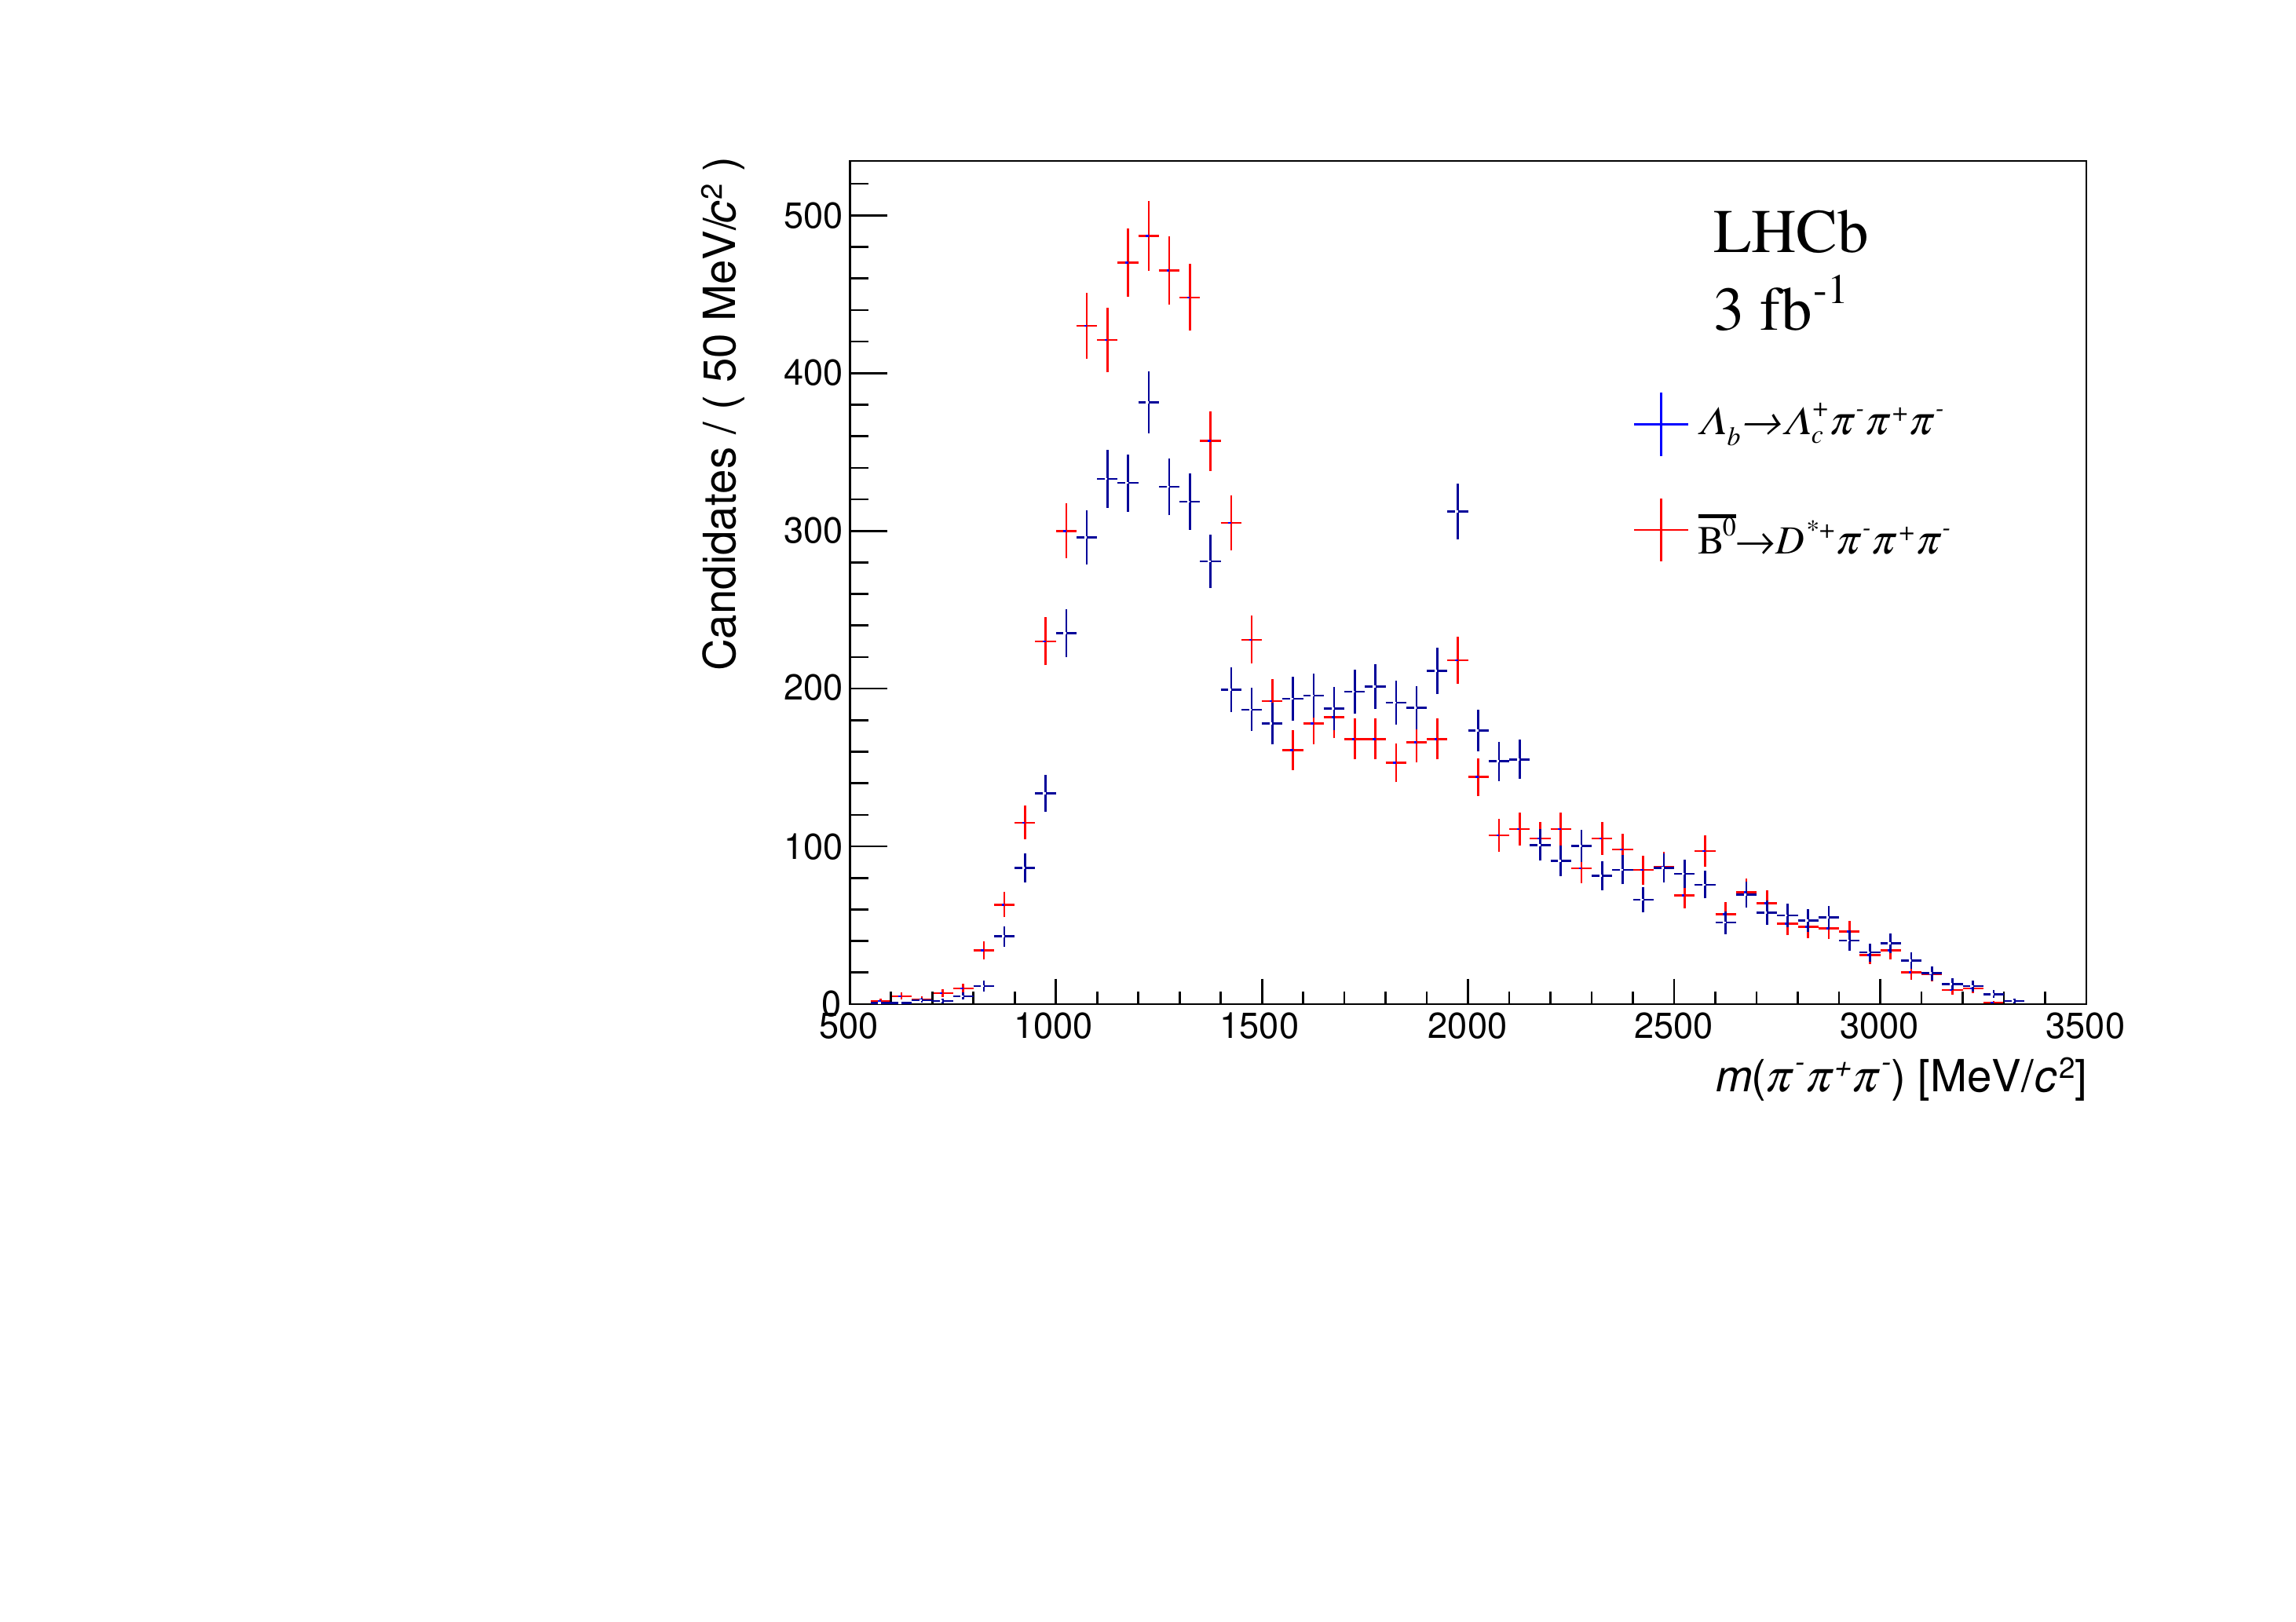}
        \caption{
    \small %captions should be a little bit smaller than main text
Distribution of the \pim\pip\pim invariant mass for all candidates in  (blue) the \mbox{\Lb\to\Lc\pim\pip\pim} channel where the \Lcstar contributions have not been removed and in (red) the  \mbox{\Bzb\to\Dstarp\pim\pip\pim} channel. The two distributions are normalised to the same area.}
  \label{figsupp:noepluch}
\end{figure}
\begin{figure}[h]
    \centering
        \includegraphics[width=0.8\textwidth]{../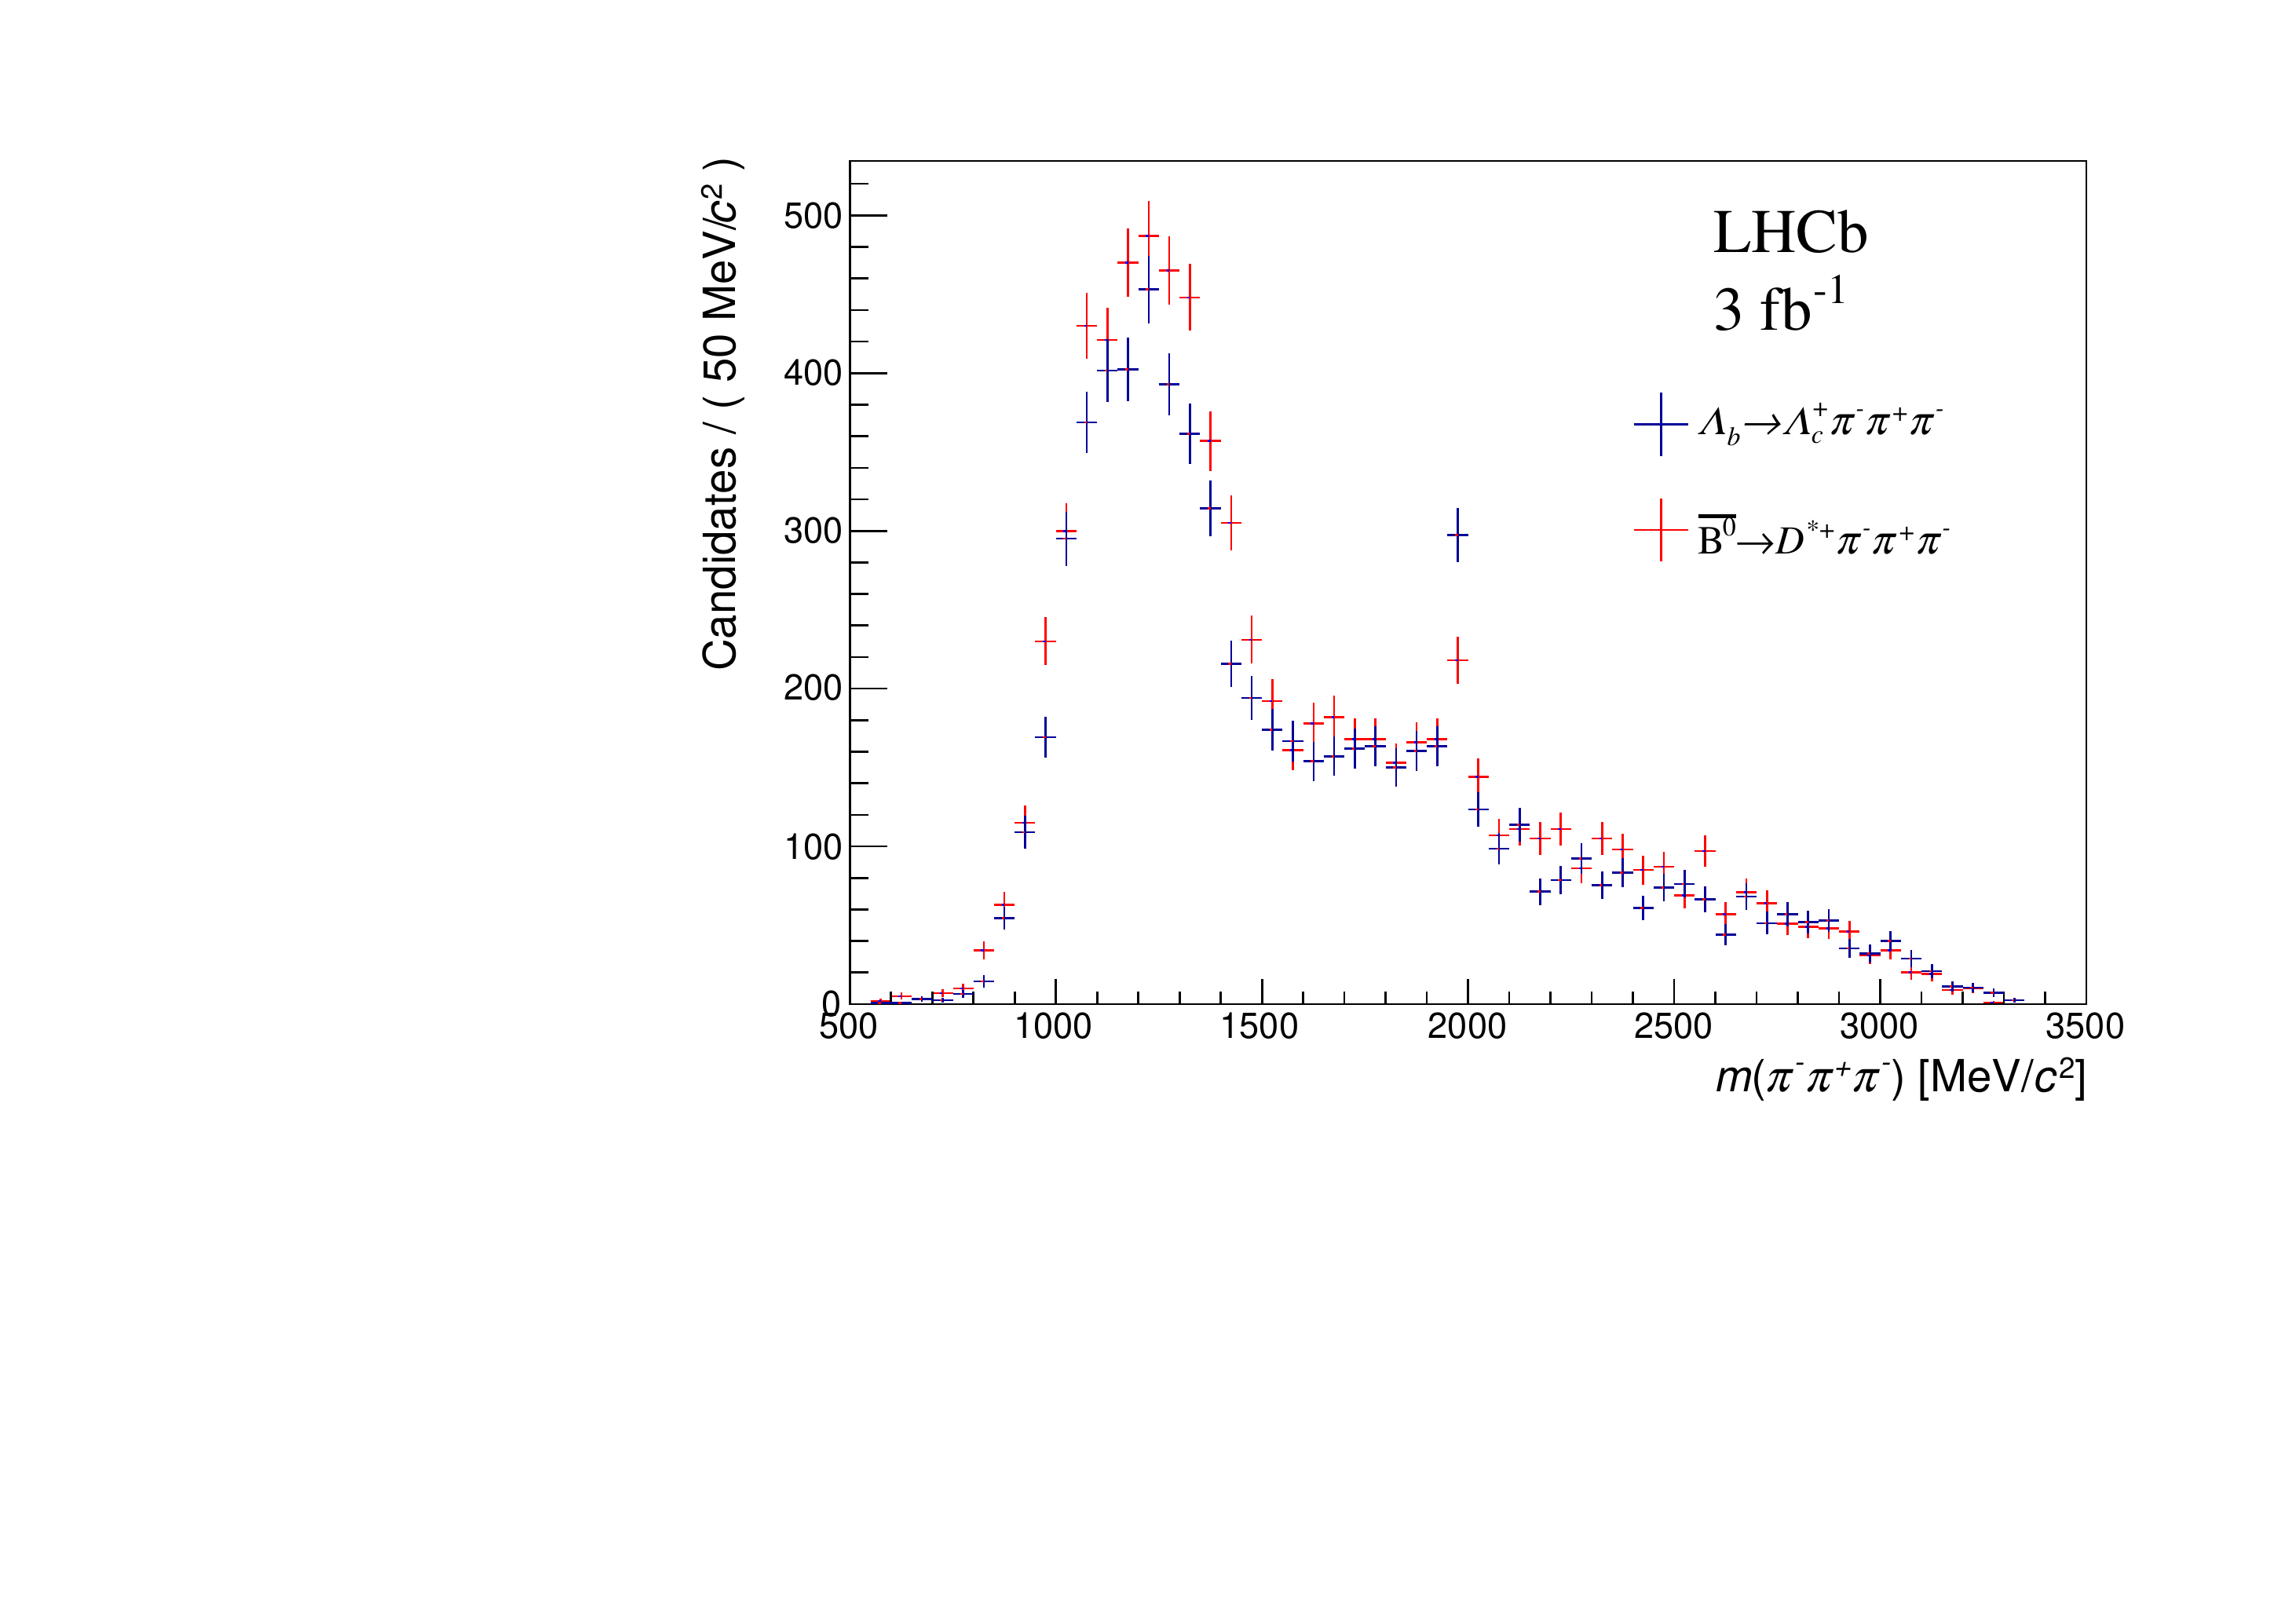}
        \caption{
    \small %captions should be a little bit smaller than main text
Distribution of the \pim\pip\pim invariant mass for all candidates in  (blue) the \mbox{\Lb\to\Lc\pim\pip\pim}  channel where the \Lcstar contributions have  been removed and in (red) the \mbox{\Bzb\to\Dstarp\pim\pip\pim} channel. The two distributions are normalised to the same area.}
  \label{figsupp:epluch}
\end{figure}
%\begin{figure}[h]
%    \centering
%        \includegraphics[width=0.8\textwidth]{../figs/Scheme_LcTauNu.png}
%        \caption{
%    \small %captions should be a little bit smaller than main text
%Schematics of the vertex topology for \Lb\to\Lc\taum\neutb events. The 5$\sigma$ inverted topology %requirement (red) is indicated. For comparison purposes, the 4$\sigma$ detachment cut (blue)  used in %the \Bzb\to\Dstarp\taum\neutb is also displayed.}
%  \label{figsupp:schema}
%\end{figure}
\begin{figure}[h]
    \centering
        \includegraphics[width=0.8\textwidth]{../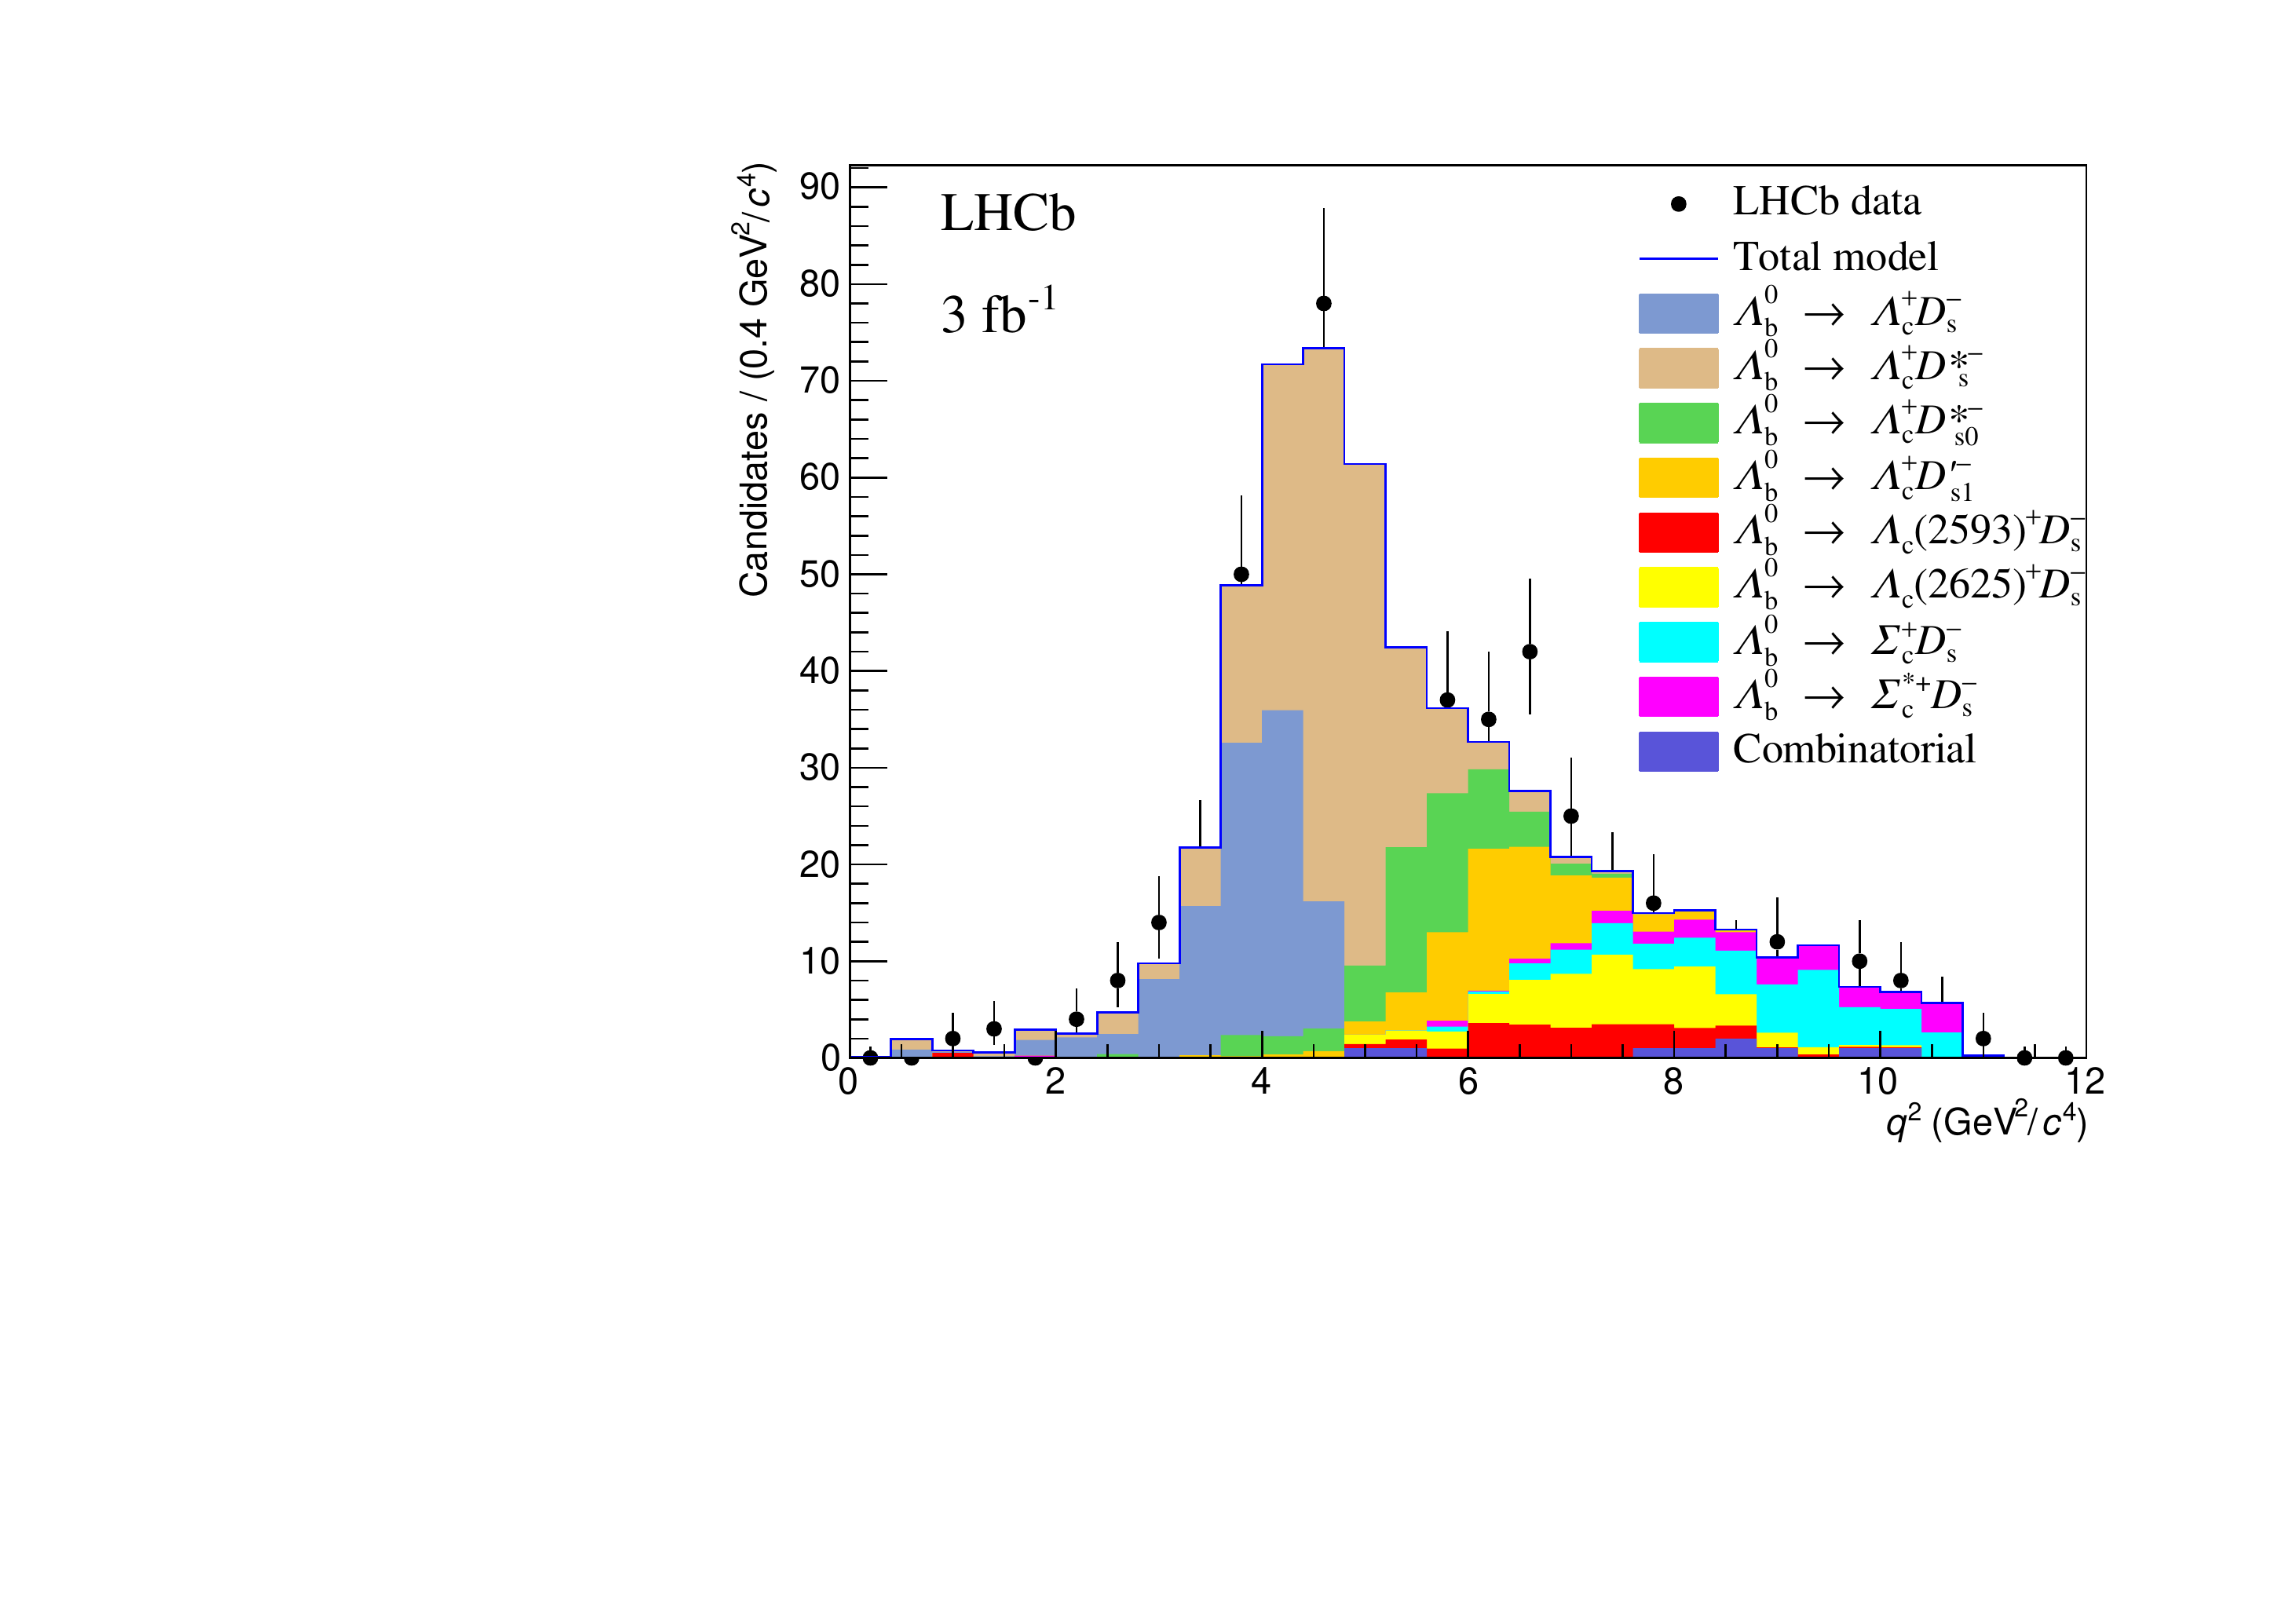}
        \caption{
    \small %captions should be a little bit smaller than main text
Distribution of \qsq for all candidates in the  $\Lc3\pion$ control sample where the mass of the 3\pion system is selected around the \Dsm mass. The rates of the various components indicated in the legend are taken for the fit results to the $\Lc3\pion$ mass fit described in the paper.}
  \label{figsupp:dsfit_q2}
\end{figure}
\begin{table}[h]
    \centering
    \footnotesize
    \begin{tabular}{lrr}
%        \toprule
        Parameter & Fit result & Constraint value \\\hline
%        \midrule
        $N_{sig}$                & $349\pm 40\ (11.8\%)$ &       \\
        $f_{\decay{\tauon}{3\pion\neu}}$ &                             & 0.78  \\
        $f_{\Lambda_c^*\tauon\neutb}$    &                             & 0.1 \\
        $N^{same}_{D^0}$                 & $80.2 \pm 8.3$              & $81.4 \pm 7.4$ \\
        $f^{v_1-v_2}_{D^0}$              & $1.3 \pm 0.7$             & \\
        $N_{D_s}$                      & $2755.9 \pm 81$           & \\
        $f_{D_s}$                        & $0.49 \pm 0.09 $          & $0.65 \pm 0.08$ \\
        $f_{D^*_{s0}}$                   & $0.0 \pm 0.012 $          & $0.28 \pm 0.12$ \\
        $f_{D^{'}_{s1}}$                 & $0.41 \pm 0.07 $          & $0.29 \pm 0.12$ \\
        $f_{\Lambda_c(2625)D_{s}^{(*)}}$   & $0.19 \pm 0.06$          & $0.22 \pm 0.09$ \\
        $f_{\Sigma_c\pion D_{s}^{(*)}}$   & $0.0\pm 0.02$          & $0.22 \pm 0.05$ \\
        $N_{D^+}$                           & $443\pm54$          &\\
        $N_{combi}$                      &                             & 40.3 \\
        $N_{\Lc}^{bkg}$                  &                             & 639 \\
        $\chi^2$                         & $256$                     &  \\
        reduced $\chi^2$ ($ndof=216$)    & $1.30$                     &  \\\hline
%        \bottomrule
    \end{tabular}
    \caption{Nominal fit results. The parameter $f_{\decay{\tauon}{3\pion\neu}}$  is the relative abundance of the  $\decay{\taum}{3\pion\neu}$ candidates wrt to all \taum candidates; $f_{\Lambda_c^*\tauon\neutb}$ is the relative yield of  \Lb\to\Lcstar\taum\neutb candidates wrt to the signal yield;   
        $N^{same}_{D^0}$ is the number of $\Lb\to\Lc\Dzb X$ candidates where the 3 pions originate from the same vertex; $f^{v_1-v_2}_{D^0}$ is the relative yield of $\Lb\to\Lc\Dzb X$ candidates where the 3 pions do not originate from the same vertex wrt to the simulation prediction; $N_{D_s}$ is the total number of $\Lb\to\Lc\Dsm(X)$ candidates; $f_{D_s}$, $f_{D^*_{s0}}$, $f_{D^{'}_{s1}}$, $f_{\Lambda_c(2625)D_{s}^{(*)}}$, $f_{\Sigma_c\pion D_{s}^{(*)}}$ are the relative yields of $\Lb\to\Lc\Dsm$, $\Lb\to\Lc D^*_{s0}$, $\Lb\to\Lc D^{'}_{s1}$, $\Lb\to\Lambda_c(2625)D_{s}^{(*)}$, $\Lb\to\Sigma_c\pion D_{s}^{(*)}$ decays wrt to that of the $\Lb\to\Lc D_s^{*-}$ channel, respectively; $N_{D^+}$ is  the yield of $\Lb\to\Lc\Dm(X)$ candidates; $N_{combi}$, $N_{\Lc}^{bkg}$ are the yields of combinatorial and misreconstructed \Lc background, respectively.}
    \label{tab:fit_results}
\end{table}
\begin{figure}[h]
    \centering
        \includegraphics[width=0.8\textwidth]{../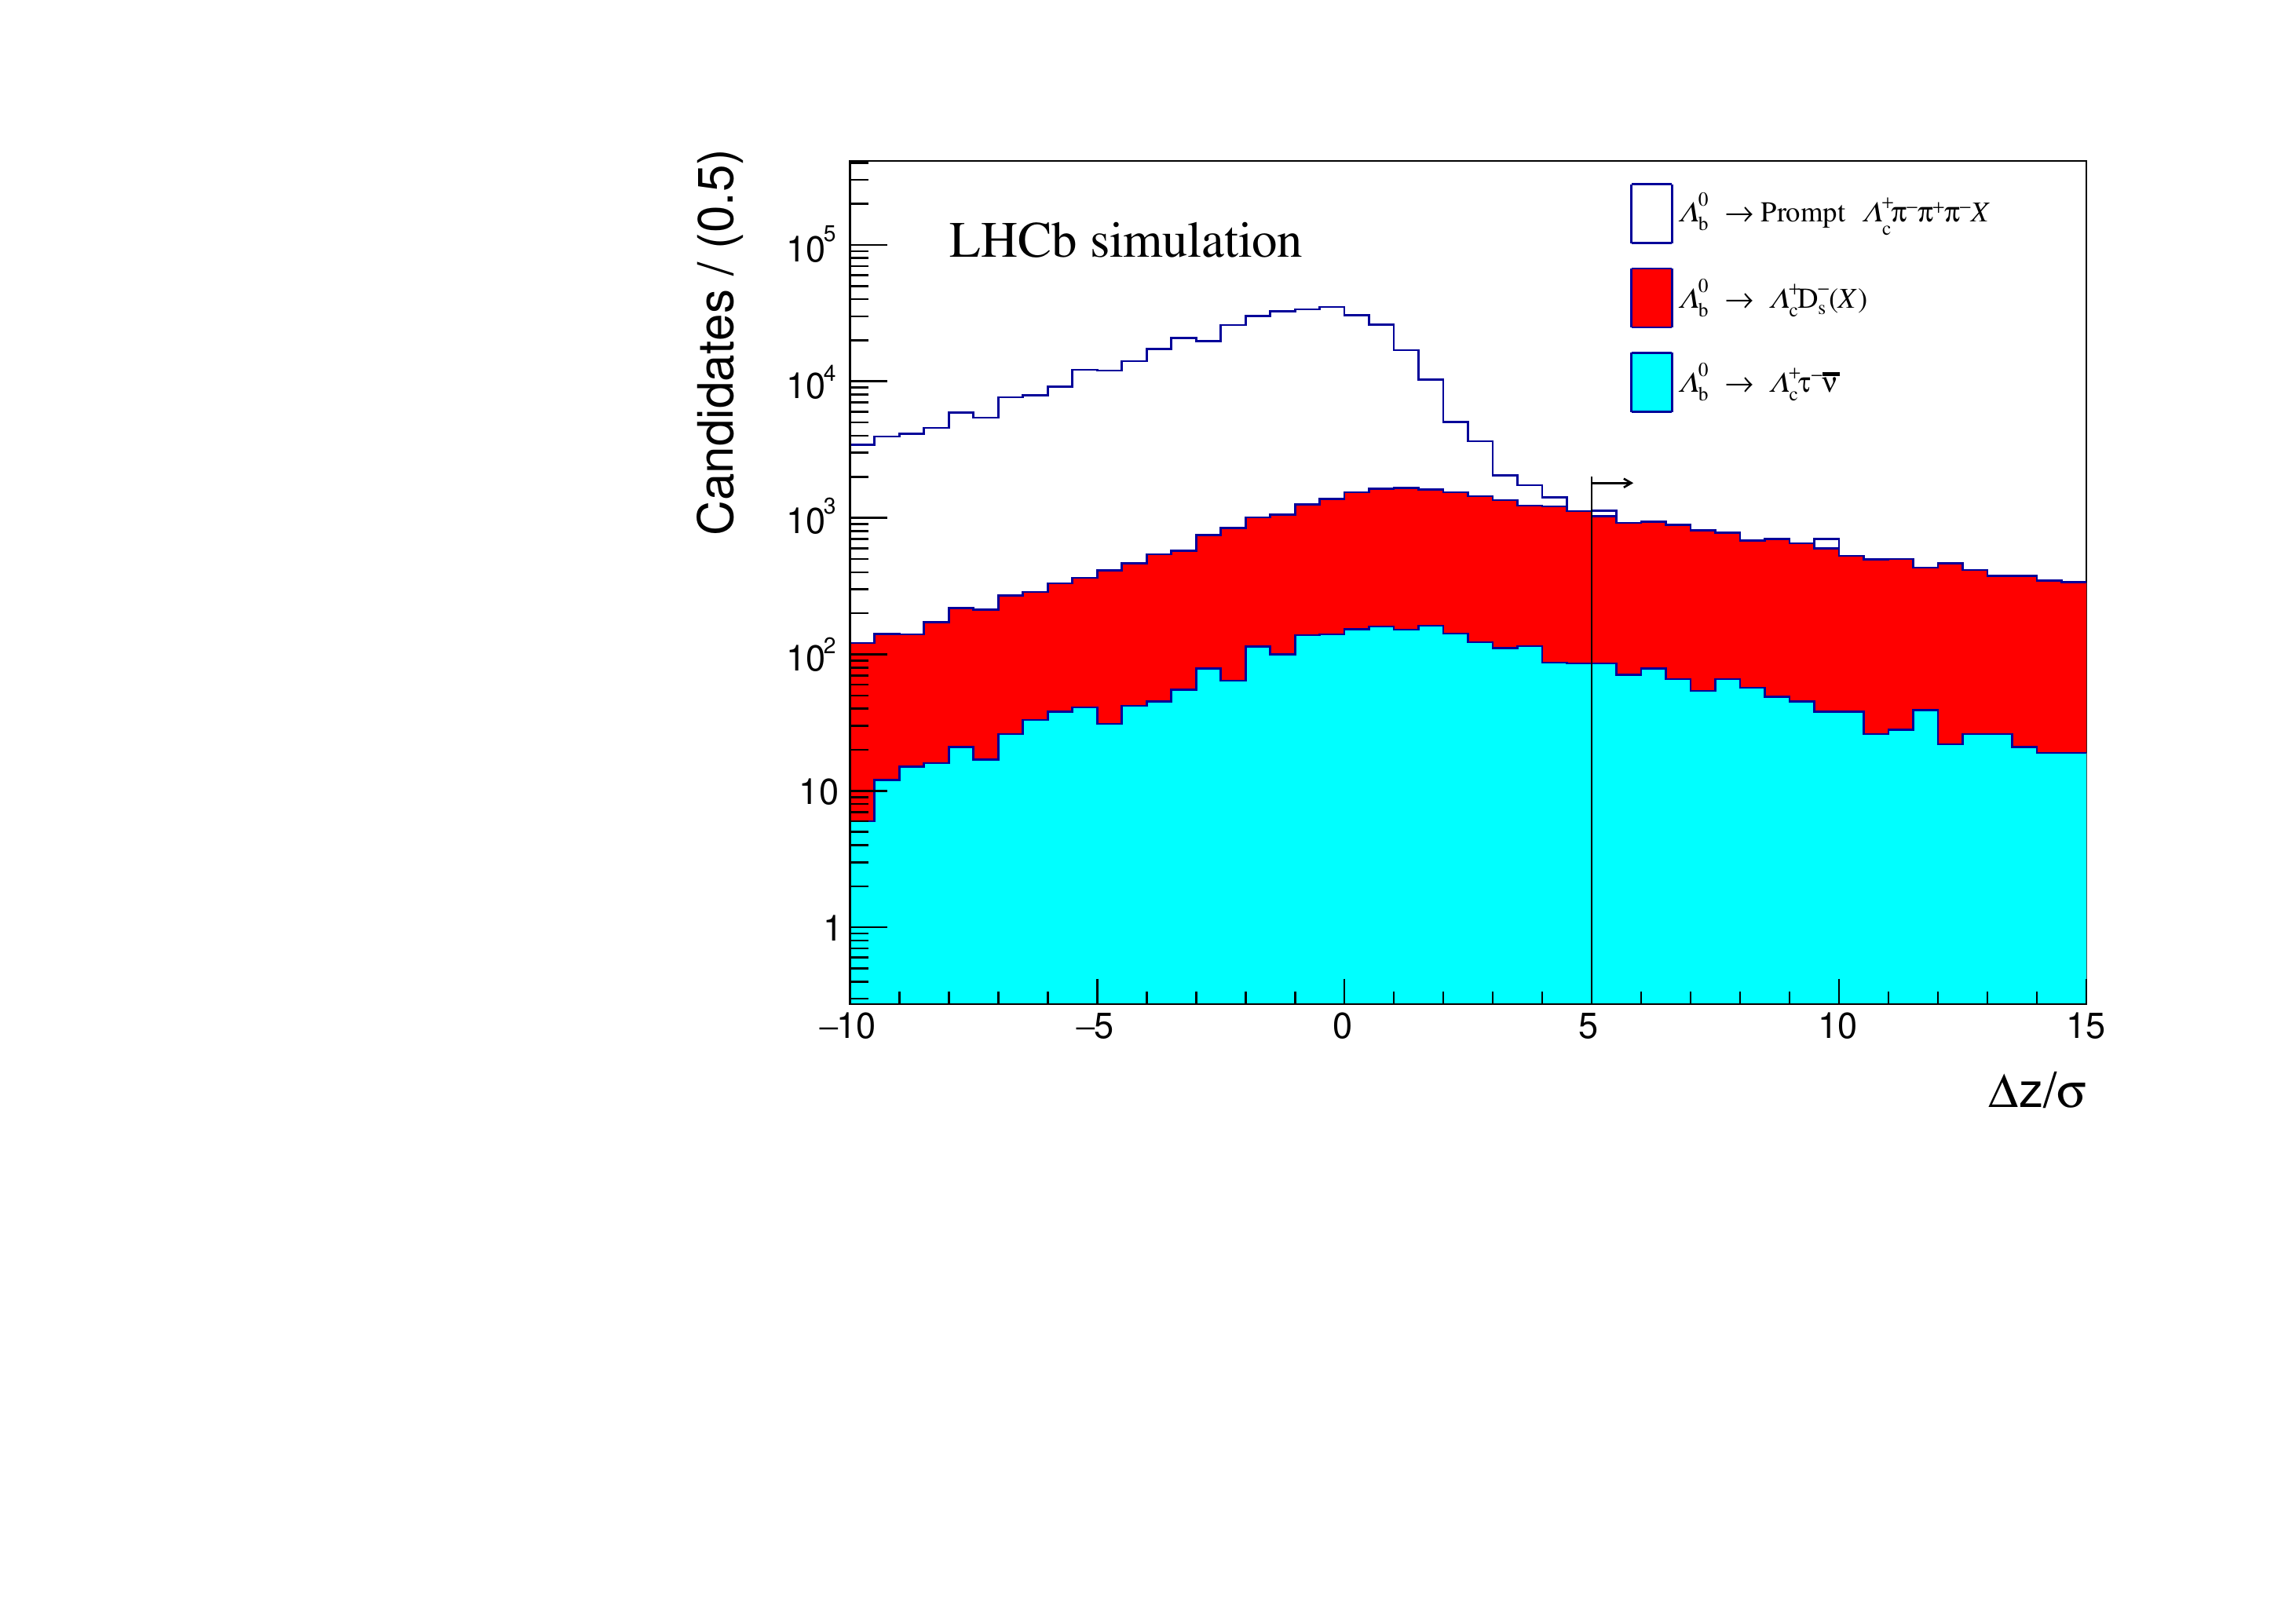}
        \caption{
    \small %captions should be a little bit smaller than main text
Distribution of the distance along the beam axis between the 3\pion and the \Lc vertices, divided by its error, for signal, $\Lb\to\Lc\Dsm(X)$ and prompt candidates, as indicated in the legend. The vertical line represents the required inverted topology requirement of 5$\sigma$.}
  \label{figsupp:deltaz}
\end{figure}
\begin{figure}[h]
    \centering
        \includegraphics[width=0.49\textwidth]{../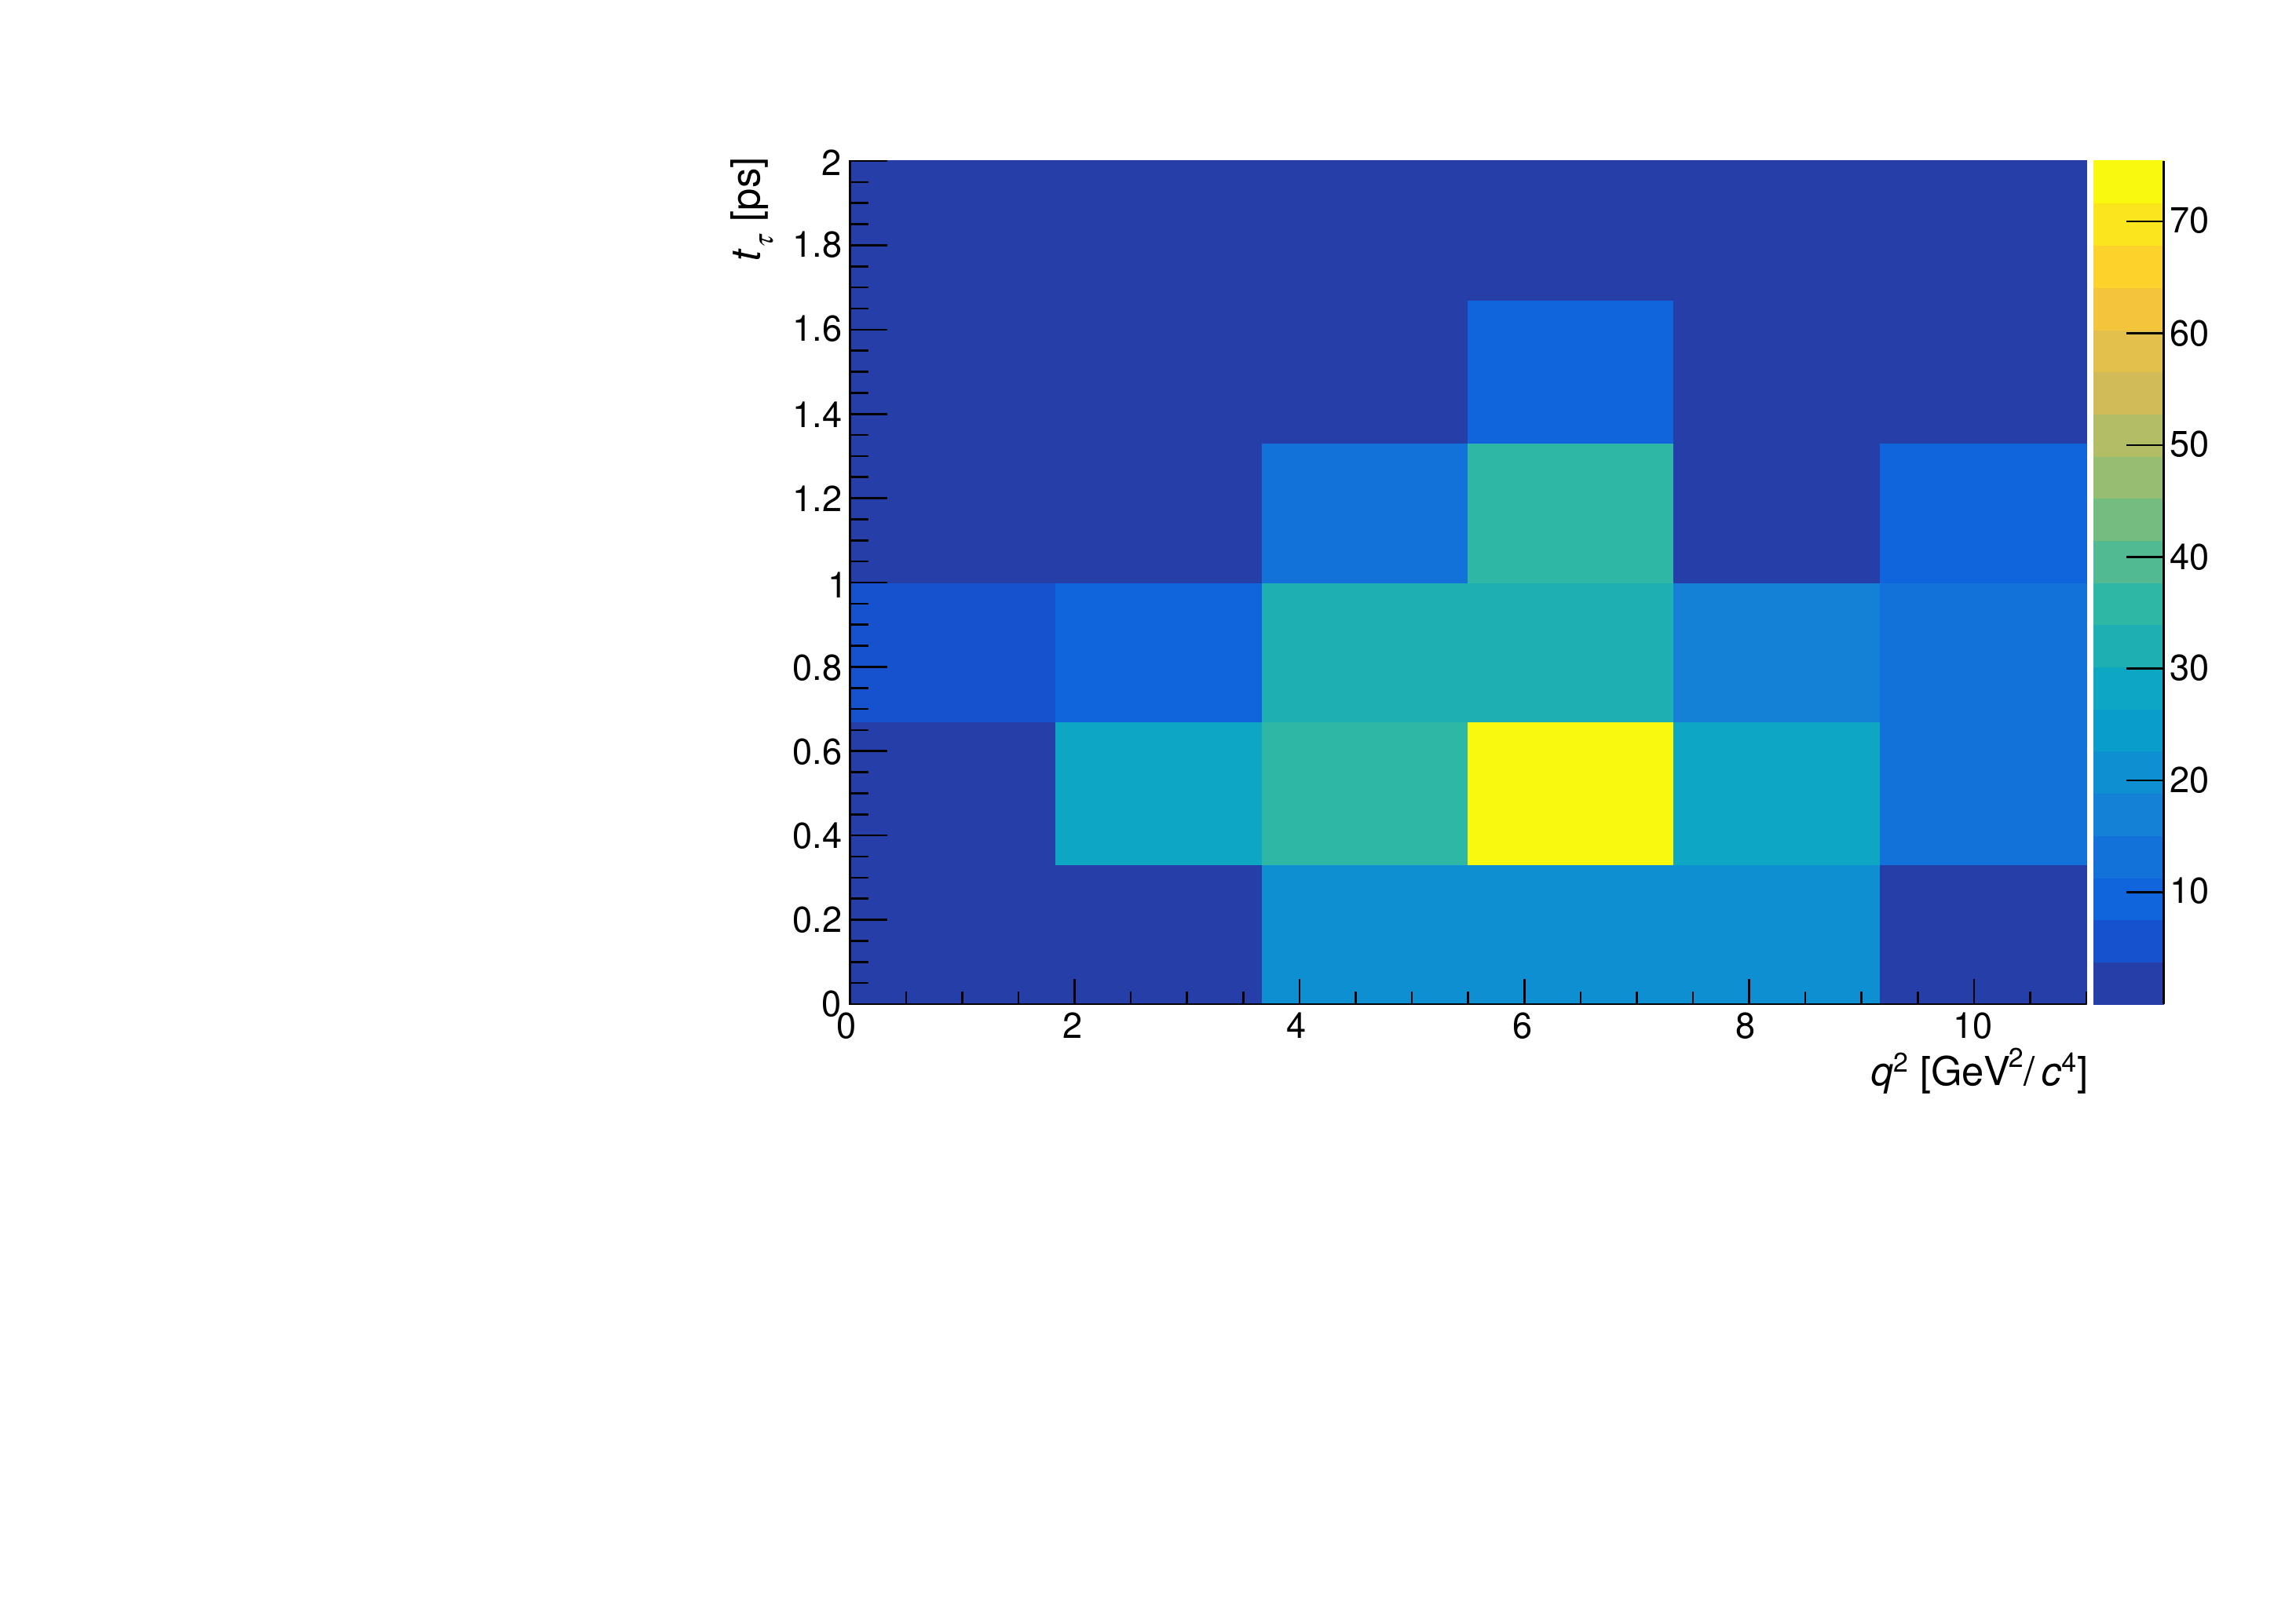}
         \includegraphics[width=0.49\textwidth]{../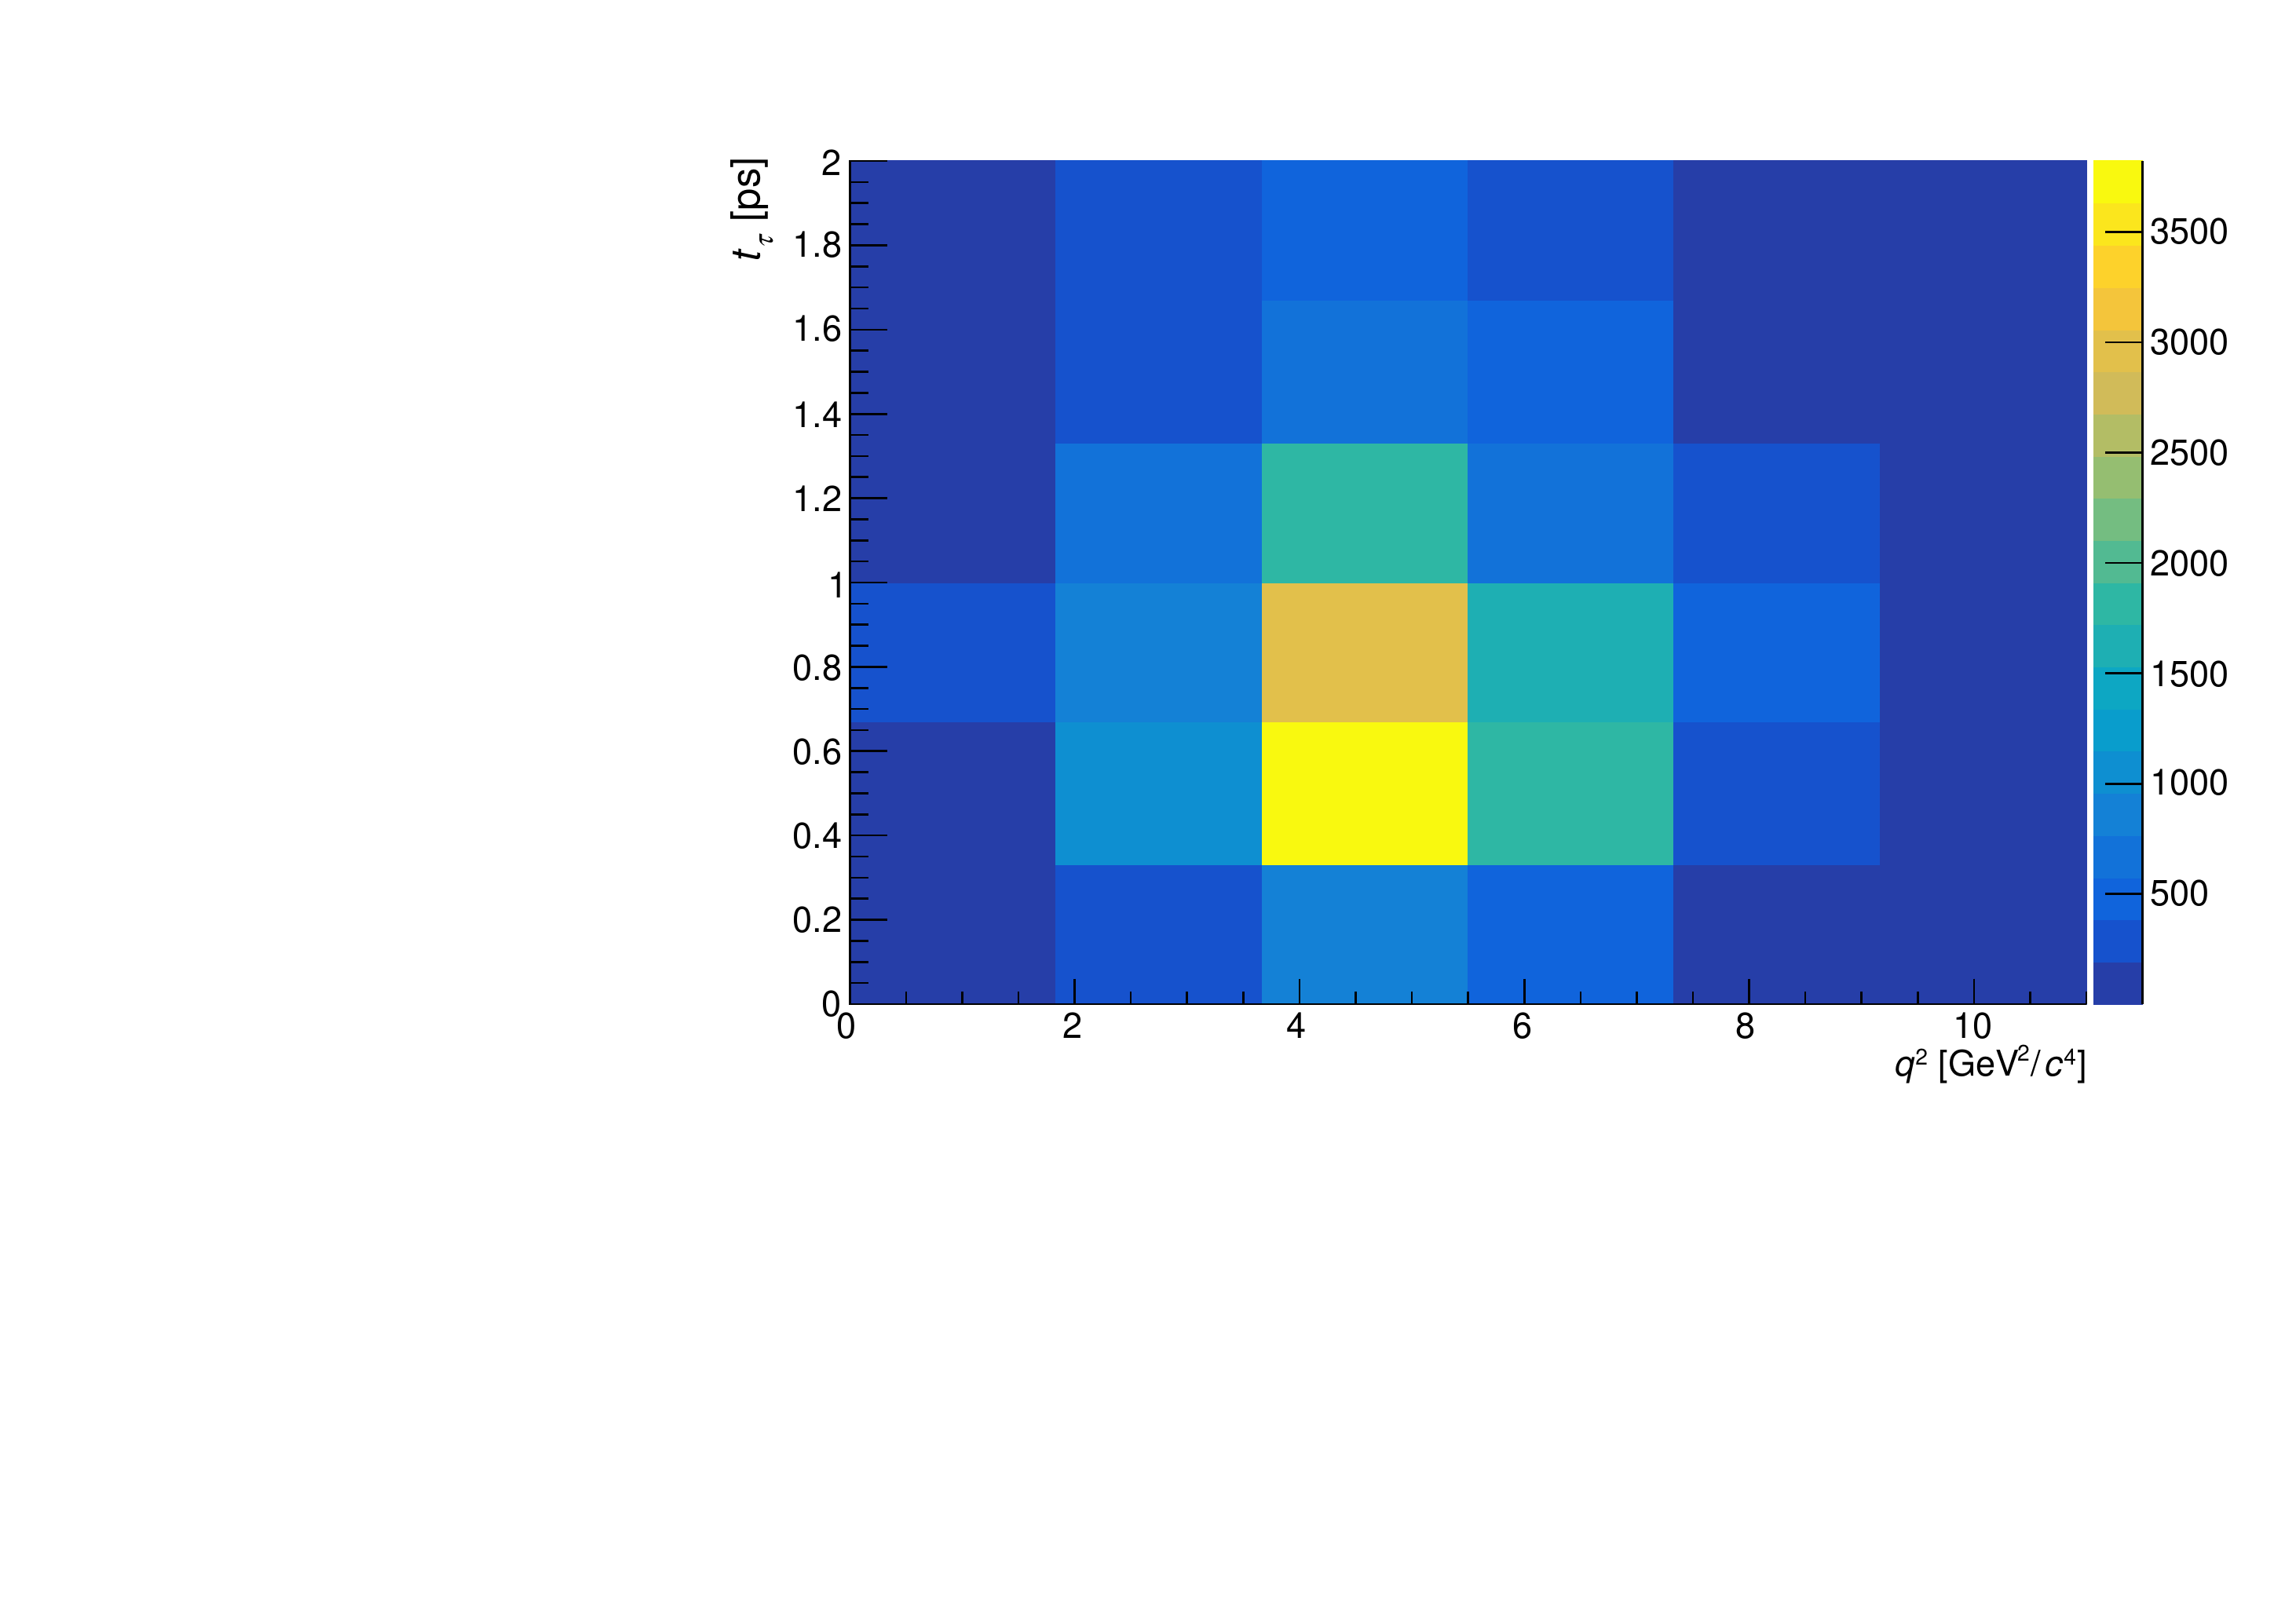}
        \caption{
    \small %captions should be a little bit smaller than main text
Distribution of  $t_\tauon$ versus \qsq variables for BDT output$<$0.66 in the simulation, for (left) \Lb\to\Lc\taum\neutb candidates and (right) $\Lb\to\Lc\Dsm(X)$ candidates.}
  \label{figsupp:tauvsq2_lowbdt}
\end{figure}
\begin{figure}[h]
    \centering
        \includegraphics[width=0.49\textwidth]{../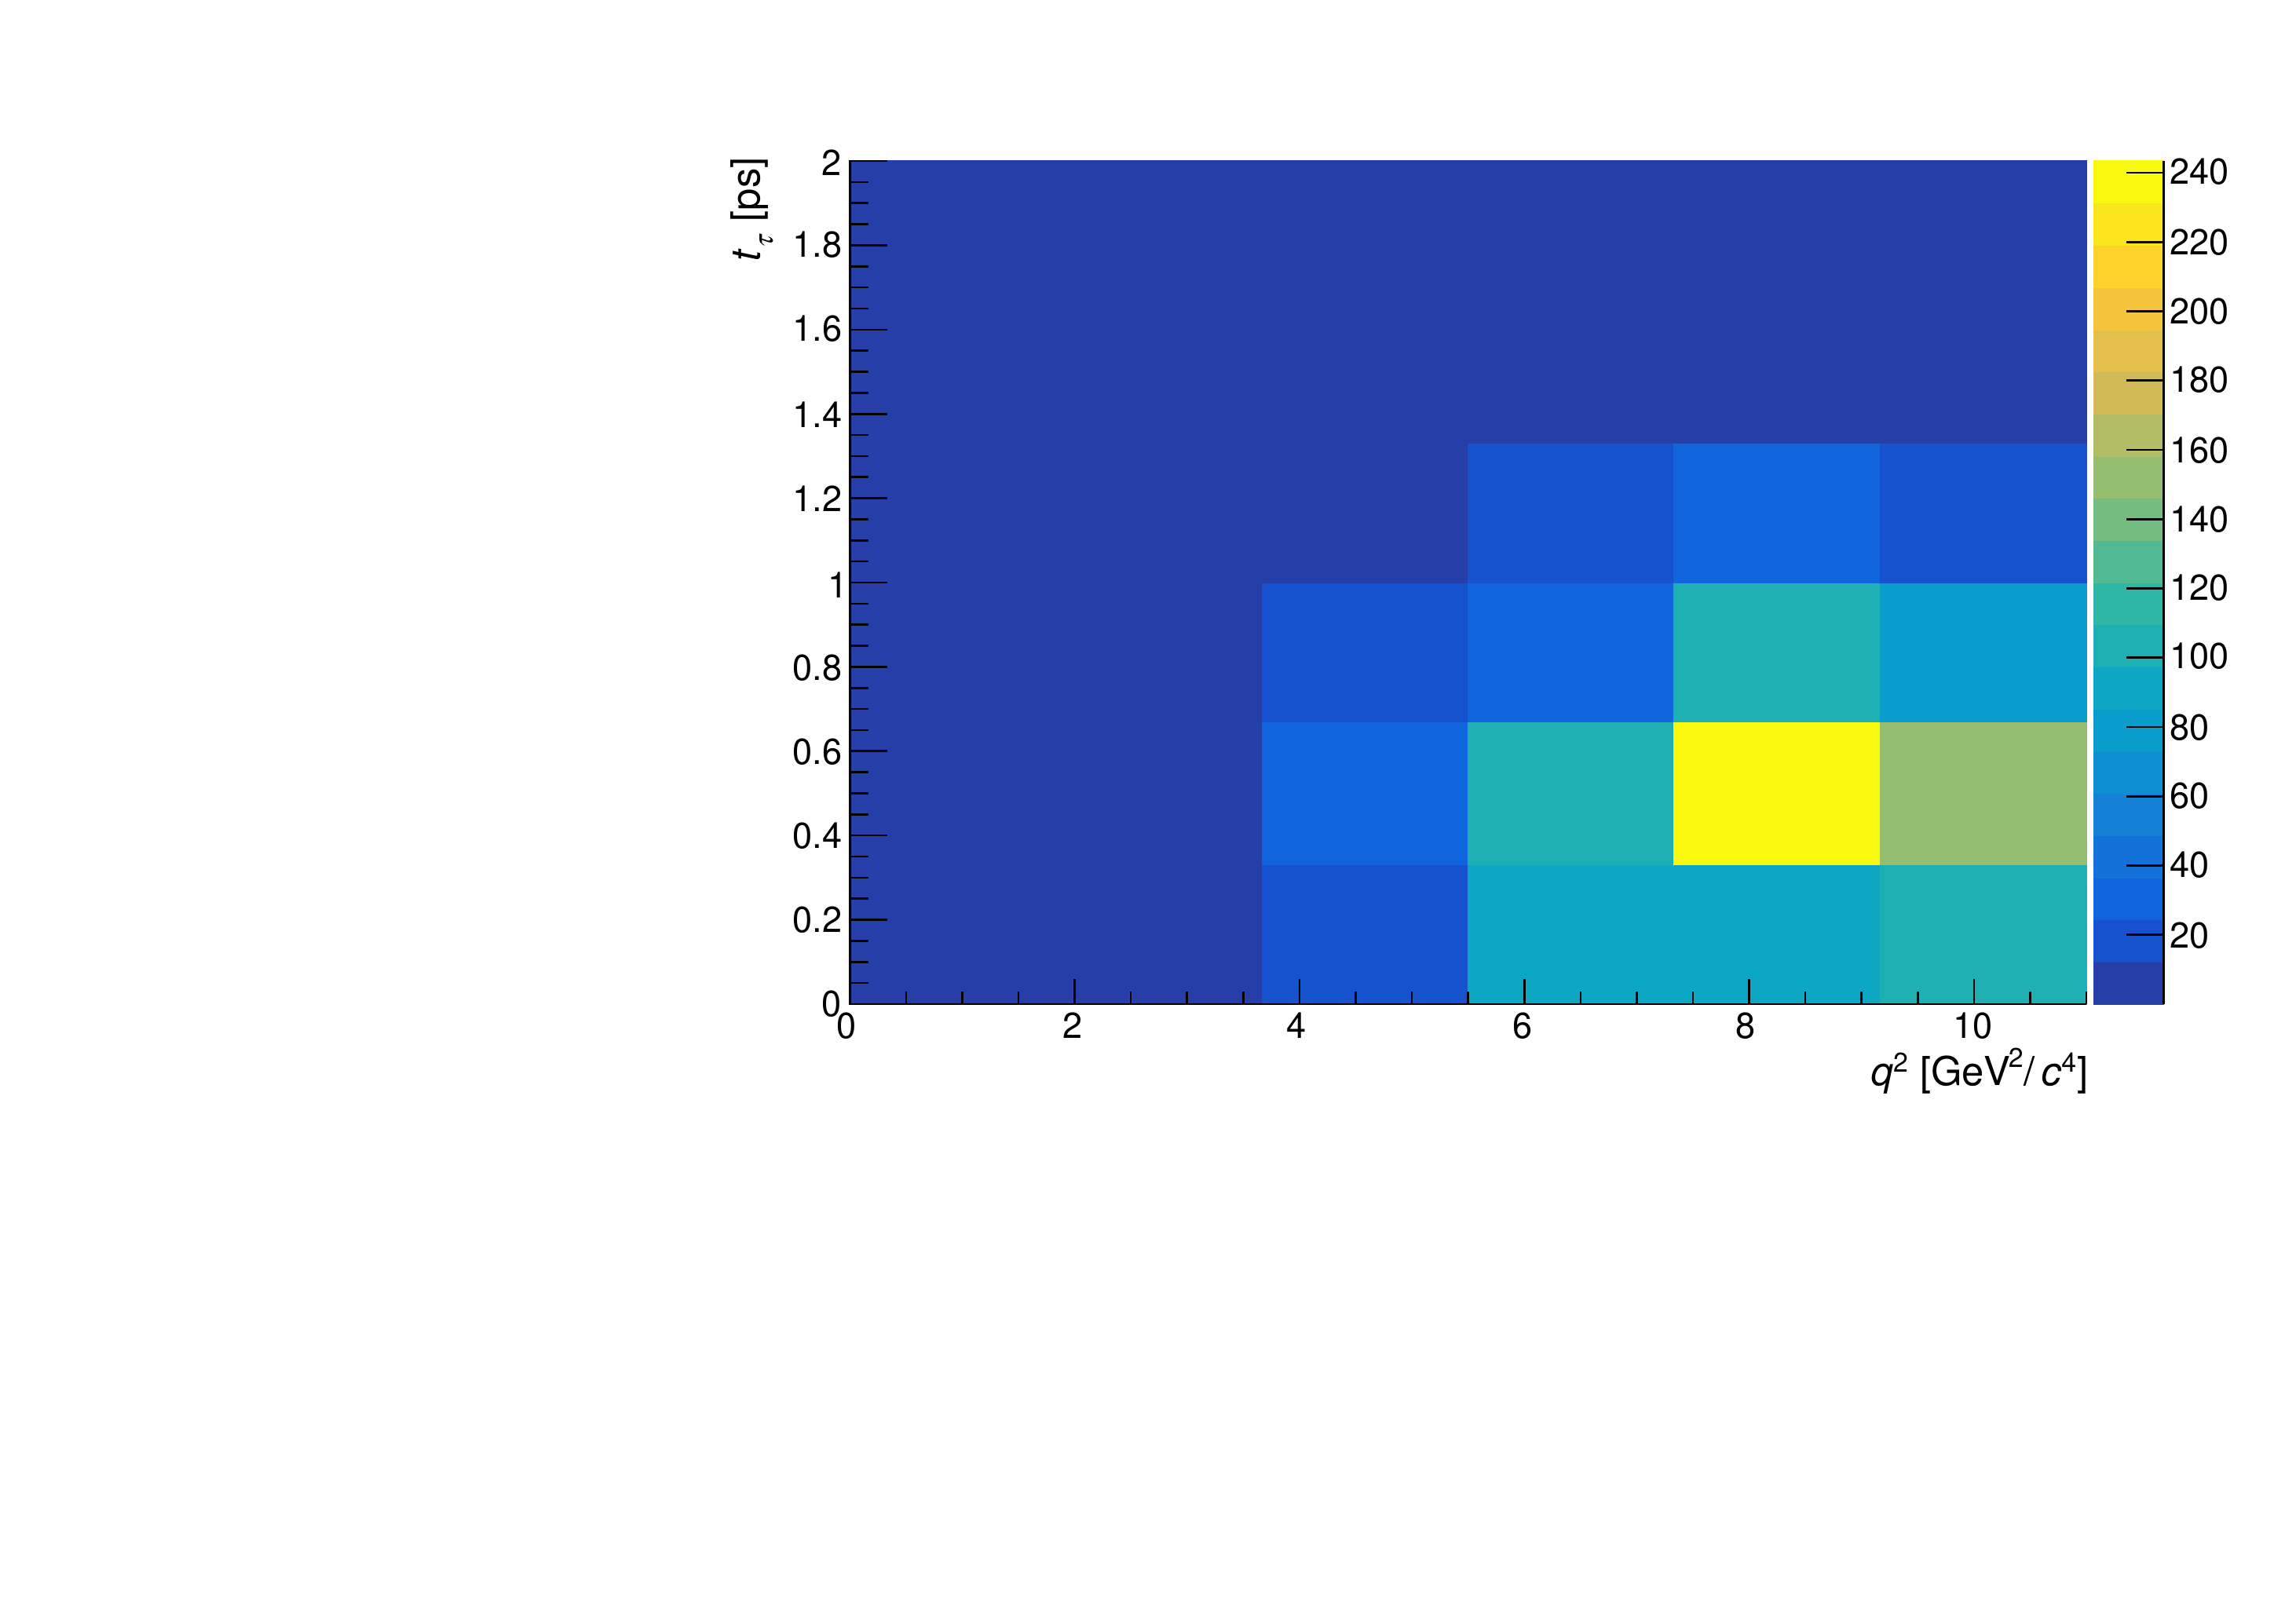}         \includegraphics[width=0.49\textwidth]{../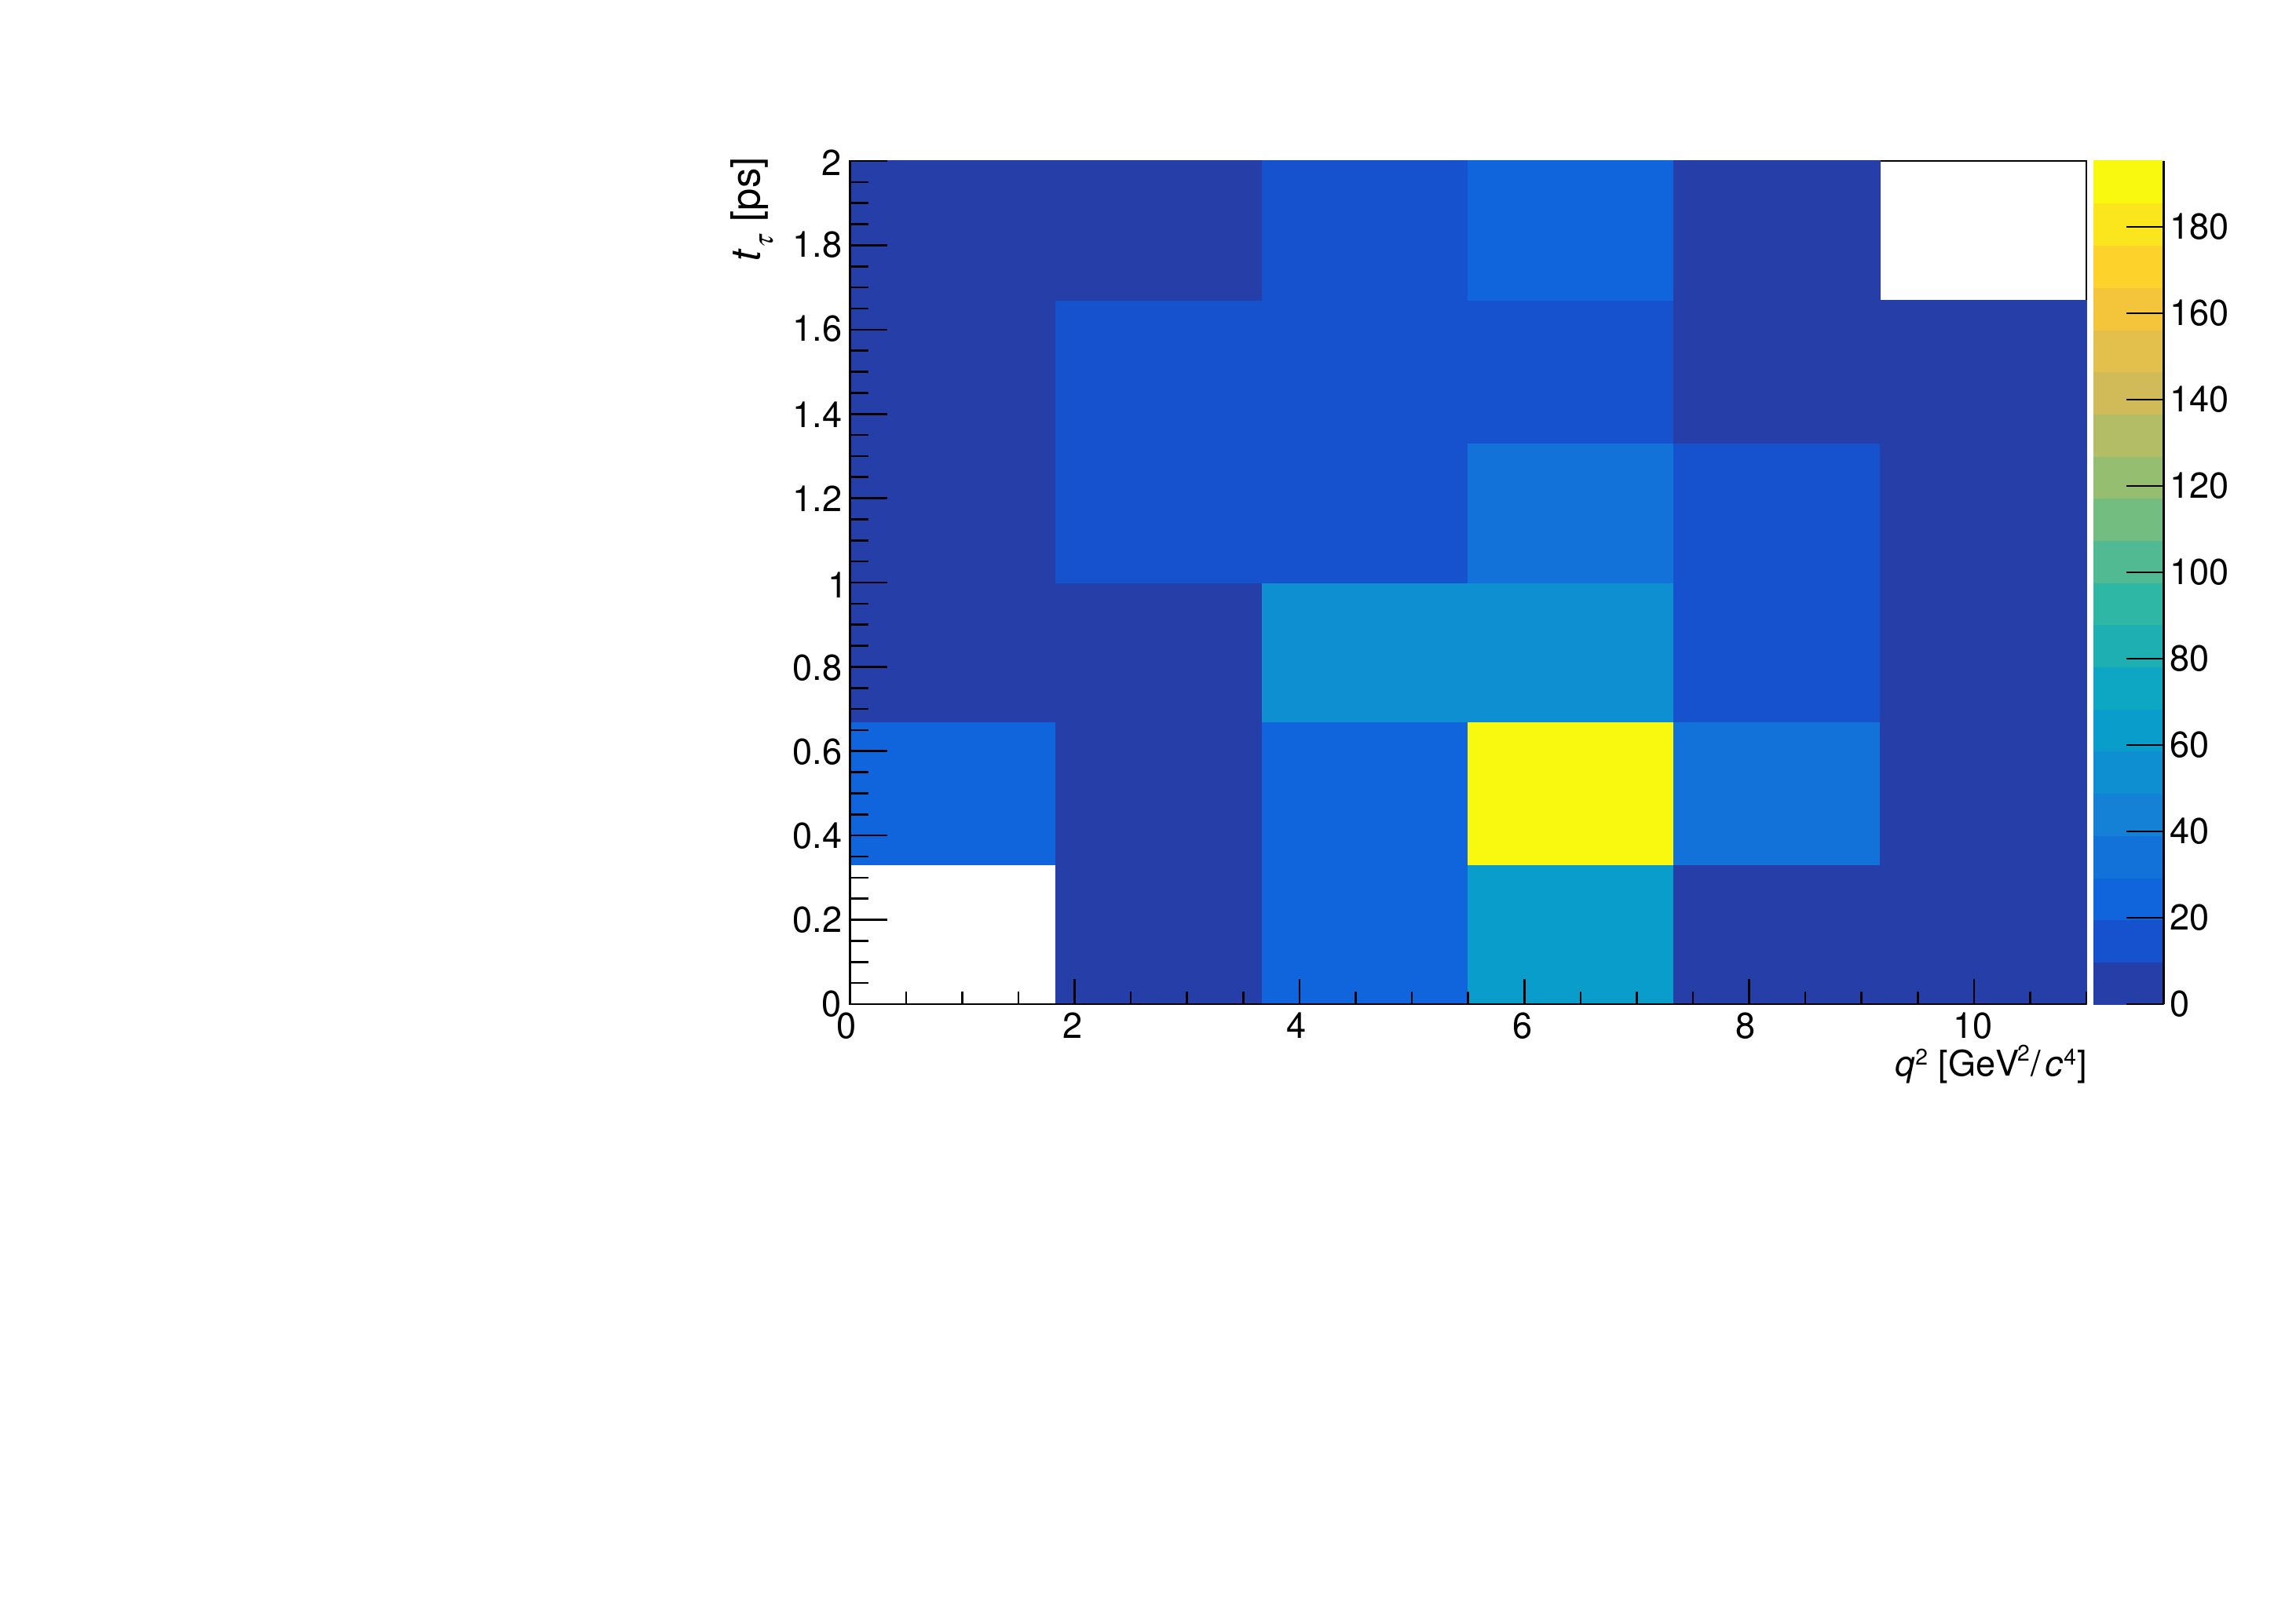}
        \caption{
    \small %captions should be a little bit smaller than main text
Distribution of  $t_\tauon$ versus \qsq variables for BDT output$>$0.66 in the simulation, for (left) \Lb\to\Lc\taum\neutb candidates and (right) $\Lb\to\Lc\Dsm(X)$ candidates.}
  \label{figsupp:tauvsq2_highbdt}
\end{figure}
