# Supplementary material for: Observation of the decay $ \Lambda_b^0\rightarrow \Lambda_c^+\tau^-\overline{\nu}_{\tau}$
Source: arXiv:2201.03497 source file (2023-03-01)
Supplement: Supplementary file 2 [file appendix.tex]

\section*{Appendix}
This Letter is appropriate for PRL journal because it is the first observation of an important $b$-hadron decay channel for which a precise prediction exists in the Standard Model framework and where physics beyond the Standard Model can play a significant role. Important results regarding the Lepton Flavour Universality, a very hot topic in particle physics, are contained therein, as well as constraints on New Physics model. The description of the analysis can be made compact, and therefore well suited to PRL, because  technical details have been described in a previous PRD publication  corresponding to  $b$-meson semitauonic decays.
